# Supplementary material for: Modelling and Simulation of an Alkaline Ni/Zn Cell
Source: arXiv:2509.05026 ancillary file (2025-09-05)
Supplement: Supplementary file 1 [file Ni_Zn_____3D_ESI.pdf]

# Modelling and Simulation of an Alkaline Ni/Zn Cell

Felix K. Schwab,<sup>\*,+,a,b</sup> Britta Doppl,<sup>+,a,b</sup> Niklas J. Herrmann,<sup>a,b</sup> Alice Boudet,<sup>d</sup> Shadi Mirhashemi,<sup>d</sup> Sylvain Brimaud,<sup>e</sup> and Birger Horstmann<sup>\*,a,b,c</sup>

<sup>\*</sup> Corresponding authors (E-mail: felix.schwab@dlr.de, birger.horstmann@dlr.de)  
<sup>+</sup> These authors contributed equally.  
<sup>a</sup> Institute of Engineering Thermodynamics - Computational Electrochemistry, German Aerospace Center (DLR), Wilhelm-Runge-Str. 10, 89081 Ulm, Germany.  
<sup>b</sup> Helmholtz Institute Ulm (HIU), Helmholtzstr. 11, 89081 Ulm, Germany.  
<sup>c</sup> Faculty of Natural Science, Ulm University, Albert-Einstein-Allee 11, 89069 Ulm, Germany.  
<sup>d</sup> SunErgy, 85-93 Boulevard Alsace-Lorraine, 93115 Rosny-sous-Bois, France.  
<sup>e</sup> Zentrum für Sonnenenergie- und Wasserstoff-Forschung Baden-Württemberg (ZSW), Helmholtzstr. 8, 89081 Ulm, Germany.

## Electronic Supplementary Information

### Contents

|                                                           |    |
|-----------------------------------------------------------|----|
| 1 Basic information                                       | 2  |
| 2 Geometry                                                | 2  |
| 3 (Micro-)Structure                                       | 4  |
| 4 Initial Conditions                                      | 5  |
| 5 Boundary Conditions                                     | 5  |
| 6 Solid Phases: Balance Equations and Material Parameters | 7  |
| 6.1 Balance Equations                                     | 7  |
| 6.2 Material Parameters                                   | 8  |
| 7 Liquid Phase: Balance Equations and Material Parameters | 9  |
| 7.1 Balance Equations                                     | 9  |
| 7.2 Material Parameters                                   | 9  |
| 8 Gas Phase: Balance Equations and Material Parameters    | 13 |
| 9 Reactions and Reaction Parameters                       | 13 |
| 10 Specific Surfaces                                      | 15 |
| 11 Pressure and Convection                                | 16 |
| 11.1 Balance Equations                                    | 16 |
| 11.2 Material Parameters                                  | 17 |
| 12 Auxiliary Results                                      | 19 |
| 12.1 Parameter sensitivity                                | 19 |
| 12.2 Shape change                                         | 20 |

## 1 Basic information

In the simulation framework used, all lengths are given in centimetres. Hence, all parametrisation is based on this unit. Following this, the standard concentration is  $c^\circ = 1 \cdot 10^{-3} \text{ mol cm}^{-3}$ . The underlying modelling approach for Ni/Zn battery cells relies on the work of Doppl<sup>1</sup>.

## 2 Geometry

The geometry and the layout of the simulation domain (see Figure S1) is based on the design of SUNERGY's Ni/Zn cell prototype. Some differences result from restrictions of the simulation software or from incomplete knowledge about the prototype. Firstly, we assume that

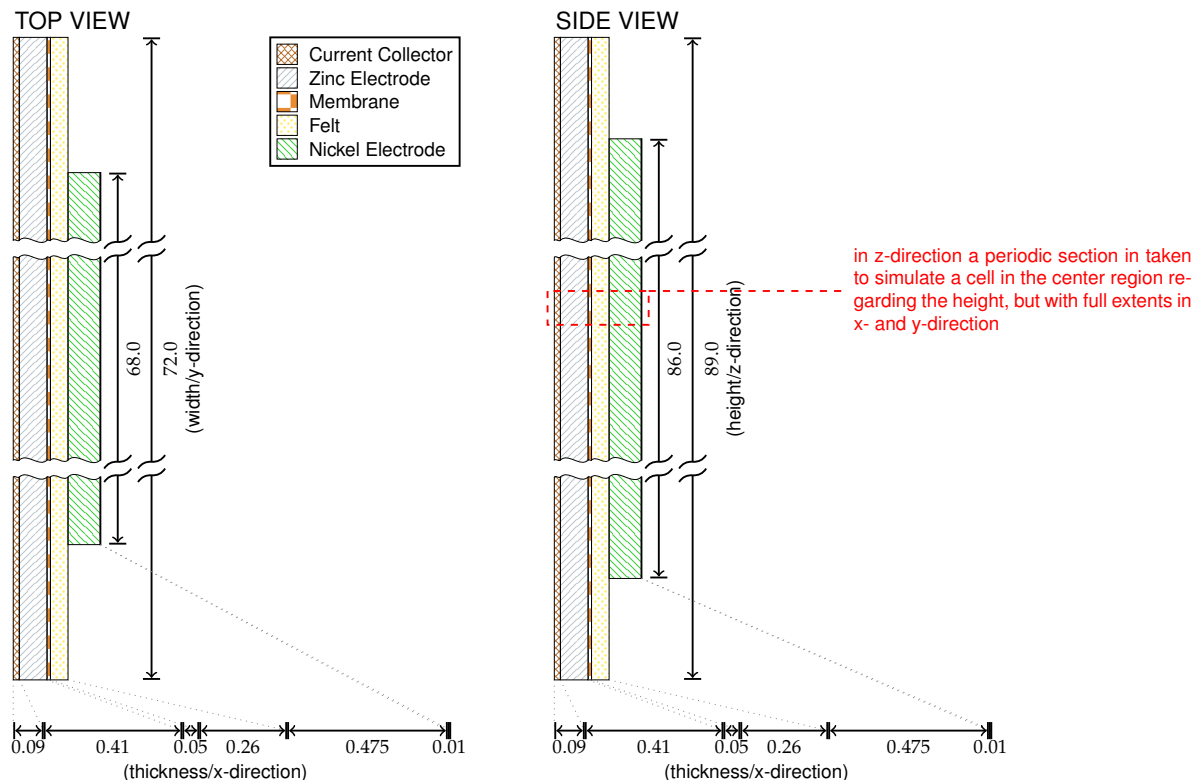

**Figure S1** Schematic depiction of top and side view of the electrochemical cell. Here, lengths are given in millimetres. The “artificial” current collector of thickness 0.01 mm next to the Ni electrode is only there, if a pseudo-1D setup is chosen.

all the different components of the cell, i.e. current collectors, electrodes, separator, felt, are aligned co-axially.

For the pseudo-1D setup, Figure S1 gives an already complete picture. An artificial current collector is attached to the Ni electrode in x-direction, because this setup is periodic in z-direction which does not allow to have tab connections at the top of the cell. Due to this, boundary conditions concerning the tab connections are also applied in x-direction.

Next, for the 3D setup, there is no artificial current collector next to the Ni electrode. Both current collectors have a small extension added in upper z-direction to mimic a tab connection for the application of the boundary conditions (cf. Figure 4 in the article). For the Ni electrode, this extension is directly attached to the electrode, as its current collector is a Ni mesh within the electrode.

The actual battery cell has a height superior to that of the electrodes. This additional height is used as an electrolyte solution reservoir and a so-called headspace, where gases ( $\text{O}_2$ ,  $\text{H}_2$ ) are collected, possibly recombined at a catalyst and/or released through a vent. These additional spaces and functionalities are not represented in the 3D model.

**Table S1** Geometrical dimensions of the single components of the electrochemical cell

| Current collector anode |      |        |                   |                                      |
|-------------------------|------|--------|-------------------|--------------------------------------|
| Variable                | Unit | Value  | Source            | Comment                              |
| thickness               | cm   | 0.0090 | Ref. <sup>2</sup> | adapted from double-sided anode      |
| width                   | cm   | 7.20   | Ref. <sup>3</sup> | assumed to have same width as anode  |
| height                  | cm   | 8.90   | Ref. <sup>3</sup> | assumed to have same height as anode |
| Anode                   |      |        |                   |                                      |
| Variable                | Unit | Value  | Source            | Comment                              |
| thickness               | cm   | 0.0410 | Ref. <sup>3</sup> | adapted from double-sided anode      |

|                                  |             |              |                     |                                                                                                                                                                                                                 |
|----------------------------------|-------------|--------------|---------------------|-----------------------------------------------------------------------------------------------------------------------------------------------------------------------------------------------------------------|
| width                            | cm          | 7.20         | Ref. <sup>3</sup>   | —                                                                                                                                                                                                               |
| height                           | cm          | 8.90         | Ref. <sup>3</sup>   | —                                                                                                                                                                                                               |
| <b>Membrane</b>                  |             |              |                     |                                                                                                                                                                                                                 |
| <b>Variable</b>                  | <b>Unit</b> | <b>Value</b> | <b>Source</b>       | <b>Comment</b>                                                                                                                                                                                                  |
| thickness                        | cm          | 0.0050       | Ref. <sup>3</sup>   | two layers of membrane with thickness 25 $\mu\text{m}$                                                                                                                                                          |
| width                            | cm          | 7.20         | Ref. <sup>3</sup>   | assumed to have same width as anode                                                                                                                                                                             |
| height                           | cm          | 8.90         | Ref. <sup>3</sup>   | assumed to have same height as anode                                                                                                                                                                            |
| <b>Felt</b>                      |             |              |                     |                                                                                                                                                                                                                 |
| <b>Variable</b>                  | <b>Unit</b> | <b>Value</b> | <b>Source</b>       | <b>Comment</b>                                                                                                                                                                                                  |
| thickness                        | cm          | 0.0260       | Ref. <sup>2</sup>   | —                                                                                                                                                                                                               |
| width                            | cm          | 7.20         | Ref. <sup>3</sup>   | assumed to have same width as anode                                                                                                                                                                             |
| height                           | cm          | 8.90         | Ref. <sup>3</sup>   | assumed to have same height as anode                                                                                                                                                                            |
| <b>Cathode</b>                   |             |              |                     |                                                                                                                                                                                                                 |
| <b>Variable</b>                  | <b>Unit</b> | <b>Value</b> | <b>Source</b>       | <b>Comment</b>                                                                                                                                                                                                  |
| thickness                        | cm          | 0.0475       | Ref. <sup>3</sup>   | adapted from double-sided cathode                                                                                                                                                                               |
| width                            | cm          | 6.80         | Ref. <sup>3</sup>   | —                                                                                                                                                                                                               |
| height                           | cm          | 8.60         | Ref. <sup>2</sup>   | —                                                                                                                                                                                                               |
| <b>Current collector cathode</b> |             |              |                     |                                                                                                                                                                                                                 |
| <b>Variable</b>                  | <b>Unit</b> | <b>Value</b> | <b>Source</b>       | <b>Comment</b>                                                                                                                                                                                                  |
| thickness                        | cm          | 0.0010       | Ref. <sup>2,3</sup> | actually, there is no current collector present; it is within the cathode in form of a nickel mesh. For modelling reasons, we attach a very thin “artificial” current collector if a pseudo-1D setup is chosen. |
| width                            | cm          | 6.80         | Ref. <sup>3</sup>   | assumed to have same width as cathode                                                                                                                                                                           |
| height                           | cm          | 8.60         | Ref. <sup>2</sup>   | assumed to have same height as cathode                                                                                                                                                                          |

The final simulation setups have some special characteristics: The space around the Ni electrode (in y- and z-direction), which accounts for the difference in size compared to the Zn electrode, is filled with felt material due to numerical reasons. Not visible in Figure S1 but done in the prototype and hence as well in the 3D setup, the Zn electrode has not only a layer of membrane towards the Ni electrode, but is entirely wrapped by it. Around all this, to represent the distance to the battery's housing, another layer of felt is added around all components. Furthermore, in terms of discretisation, a non-equidistant grid is used to reduce computational costs. All setups discretise the representative active material particles in the Ni electrode, where the radial solid diffusion process of proton insertion is taking place, by five equidistant grid points. The associated voxel size depends on the chosen particle size, which may be found in Table S3. Further details for both, the pseudo-1D and the 3D setup, are given in Table S2 and Figure S2.

**Table S2** Discretisation of the simulation domains. All distances are given in centimetres

| <b>pseudo-1D (18 × 3 × 3)</b> |           |           |           |           |           |           |           |           |           |
|-------------------------------|-----------|-----------|-----------|-----------|-----------|-----------|-----------|-----------|-----------|
| <b>Voxel No.</b>              | <b>1</b>  | <b>2</b>  | <b>3</b>  | <b>4</b>  | <b>5</b>  | <b>6</b>  | <b>7</b>  | <b>8</b>  | <b>9</b>  |
| $\Delta x$                    | 0.009000  | 0.006833  | 0.006833  | 0.006833  | 0.006833  | 0.006833  | 0.006833  | 0.005000  | 0.008667  |
| $\Delta y$                    | 0.200000  | 6.800000  | 0.200000  | —         | —         | —         | —         | —         | —         |
| $\Delta z$                    | 0.050000  | 0.050000  | 0.050000  | —         | —         | —         | —         | —         | —         |
|                               | <b>10</b> | <b>11</b> | <b>12</b> | <b>13</b> | <b>14</b> | <b>15</b> | <b>16</b> | <b>17</b> | <b>18</b> |
|                               | 0.008667  | 0.008667  | 0.007917  | 0.007917  | 0.007917  | 0.007917  | 0.007917  | 0.007917  | 0.001000  |
|                               | —         | —         | —         | —         | —         | —         | —         | —         | —         |
|                               | —         | —         | —         | —         | —         | —         | —         | —         | —         |
| <b>3D (13 × 21 × 23)</b>      |           |           |           |           |           |           |           |           |           |
| <b>Voxel No.</b>              | <b>1</b>  | <b>2</b>  | <b>3</b>  | <b>4</b>  | <b>5</b>  | <b>6</b>  | <b>7</b>  | <b>8</b>  | <b>9</b>  |
| $\Delta x$                    | 0.009000  | 0.010250  | 0.010250  | 0.010250  | 0.010250  | 0.005000  | 0.013000  | 0.013000  | 0.010000  |
| $\Delta y$                    | 0.050000  | 0.005000  | 0.050000  | 0.050000  | 0.050000  | 0.050000  | 0.300000  | 0.600000  | 0.900000  |
| $\Delta z$                    | 0.050000  | 0.005000  | 0.037500  | 0.037500  | 0.037500  | 0.037500  | 0.300000  | 0.600000  | 0.900000  |
|                               | <b>10</b> | <b>11</b> | <b>12</b> | <b>13</b> | <b>14</b> | <b>15</b> | <b>16</b> | <b>17</b> | <b>18</b> |
|                               | 0.010000  | 0.010000  | 0.010000  | 0.007500  | —         | —         | —         | —         | —         |
|                               | 1.000000  | 1.200000  | 1.000000  | 0.900000  | 0.600000  | 0.300000  | 0.050000  | 0.050000  | 0.050000  |
|                               | 0.900000  | 1.000000  | 1.200000  | 1.000000  | 0.900000  | 0.900000  | 0.600000  | 0.300000  | 0.037500  |
|                               | <b>19</b> | <b>20</b> | <b>21</b> | <b>22</b> | <b>23</b> |           |           |           |           |

|          |          |          |          |          |
|----------|----------|----------|----------|----------|
| 0.050000 | 0.005000 | 0.050000 | —        | —        |
| 0.037500 | 0.037500 | 0.037500 | 0.005000 | 0.050000 |

### 3 (Micro-)Structure

The volume fractions used here are  $\varepsilon^P$  (passive material; e.g. binder and other electrode constituents not participating in reactions),  $\varepsilon^{Zn}$  (zinc),  $\varepsilon^{ZnO}$  (zinc oxide),  $\varepsilon^{ca}$  (cathode active material, i.e.  $\beta$ -NiO(OH)/ $\beta$ -Ni(OH)<sub>2</sub>). The respective pore volume fraction (i.e. porosity) is calculated via  $\varepsilon^{pore} = 1 - \sum_{\alpha} \varepsilon^{\alpha}$ , with  $\alpha$  including all locally present solid volume fractions. The total pore space consists of the liquid and gas volume fractions,  $\varepsilon^{pore} = \varepsilon^l + \varepsilon^g$ . The tortuosity of liquid and solid phase,  $\tau^l$  and  $\tau^s$ , respectively, i.e. the scaling factor for the pathway through the porous microstructure in the liquid and solid phase, respectively, is approximated by the simple assumptions

$$\tau^l = \frac{1}{\sqrt{\varepsilon^l}} \text{ and } \tau^s = \frac{1}{\sqrt{\varepsilon^s}}, \quad (1)$$

where  $\varepsilon^s = \sum_{\alpha} \varepsilon^{\alpha}$  with, as previously,  $\alpha$  including all locally present solid volume fractions. The volume fractions of zinc and zinc oxide represents the respective initial volume fraction.

The zinc oxide is precipitated in the form of a shell around the zinc particles in the negative electrode. Experiments stress, that this shell (in the case of ZnO type-I) is porous<sup>4,5</sup>. The corresponding volume fraction is denominated by  $\varepsilon^{ZnO-L}$ , and the Bruggeman coefficient of the pores in the shell is  $\beta^{ZnO-L}$ .

The zinc electrode consists of zinc particles, and the nickel electrode of NiO(OH)/Ni(OH)<sub>2</sub> particles, which are assumed to be dense and with negligible porosity.

A gas phase does exist to balance the pressure, and through the electrolyte solution reservoir there is always enough electrolyte solution to perfectly fill the remaining pore volume. We assume an initial volume fraction of  $\varepsilon^g = 0.2 \cdot \varepsilon^{pore}$  for this implicit gas phase.

**Table S3** Microstructural details of the single components of the electrochemical cell

| Current collector anode |      |                    |                       |                                                                                            |
|-------------------------|------|--------------------|-----------------------|--------------------------------------------------------------------------------------------|
| Variable                | Unit | Value              | Source                | Comment                                                                                    |
| $\varepsilon^P$         | -    | 1.00               | —                     | pure copper                                                                                |
| Anode                   |      |                    |                       |                                                                                            |
| Variable                | Unit | Value              | Source                | Comment                                                                                    |
| $\varepsilon^P$         | -    | 0.1750             | Ref. <sup>2,3,6</sup> | mixture of binder and additives, e.g. Ca(OH) <sub>2</sub>                                  |
| $\varepsilon^{Zn}$      | -    | 0.1000             | Ref. <sup>3,6</sup>   | —                                                                                          |
| $\varepsilon^{ZnO}$     | -    | 0.1500             | Ref. <sup>3,6</sup>   | —                                                                                          |
| $\varepsilon^{pore}$    | -    | 0.5750             | Ref. <sup>6</sup>     | —                                                                                          |
| $\tau^i$                | -    | (1)                | —                     | $i = \{l, s\}$ , assumption based on Bruggeman coefficient $\beta = 1.5$                   |
| $r^{Zn}$                | cm   | 0.0075             | Ref. <sup>3</sup>     | calculated average (initial) Zn particle radius based on experimental data                 |
| $\varepsilon^{ZnO-L}$   | -    | 0.72               | Ref. <sup>4</sup>     | for 6 M KOH                                                                                |
| $\beta^{ZnO-L}$         | -    | 1.75               | —                     | estimated                                                                                  |
| Membrane                |      |                    |                       |                                                                                            |
| Variable                | Unit | Value              | Source                | Comment                                                                                    |
| $\varepsilon^P$         | -    | 0.64               | Ref. <sup>2</sup>     | —                                                                                          |
| $\varepsilon^{pore}$    | -    | 0.36               | Ref. <sup>2</sup>     | pore space filled by electrolyte solution and gas phase                                    |
| $\tau^i$                | -    | (1)                | —                     | $i = \{l, s\}$ , assumption based on Bruggeman coefficient $\beta = 1.5$                   |
| $d^{pore}$              | cm   | $37 \cdot 10^{-7}$ | Ref. <sup>2,7</sup>   | experimentally determined pore size, polypropylene membrane                                |
| Felt                    |      |                    |                       |                                                                                            |
| Variable                | Unit | Value              | Source                | Comment                                                                                    |
| $\varepsilon^P$         | -    | 0.06               | Ref. <sup>2</sup>     | —                                                                                          |
| $\varepsilon^{pore}$    | -    | 0.94               | Ref. <sup>2</sup>     | pore space filled by electrolyte solution and gas phase                                    |
| $\tau^i$                | -    | (1)                | —                     | $i = \{l, s\}$ , assumption based on Bruggeman coefficient $\beta = 1.5$                   |
| $r^{fibre}$             | cm   | $25 \cdot 10^{-4}$ | Ref. <sup>2</sup>     | material is polyolefine; here, assumption of polypropylene fibres (cf. Ref. <sup>8</sup> ) |
| Cathode                 |      |                    |                       |                                                                                            |
| Variable                | Unit | Value              | Source                | Comment                                                                                    |
| $\varepsilon^P$         | -    | 0.175              | Ref. <sup>2</sup>     | nickel mesh, binder and additives                                                          |
| $\varepsilon^{ca}$      | -    | 0.304              | Ref. <sup>2</sup>     | —                                                                                          |

|                                  |             |              |                     |                                                                                                                                |
|----------------------------------|-------------|--------------|---------------------|--------------------------------------------------------------------------------------------------------------------------------|
| $\varepsilon^{\text{pore}}$      | -           | 0.525        | Ref. <sup>2,6</sup> | pore space filled by electrolyte solution and gas phase; experimentally determined; further corrections due to additional data |
| $\tau^i$                         | -           | (1)          | —                   | $i = \{l, s\}$ , assumption based on Bruggeman coefficient $\beta = 1.5$                                                       |
| $r^{\text{Ni(OH)}_2}$            | cm          | 0.00115      | Ref. <sup>3</sup>   | calculated average NiO(OH)/Ni(OH) <sub>2</sub> particle radius                                                                 |
| <b>Current collector cathode</b> |             |              |                     |                                                                                                                                |
| <b>Variable</b>                  | <b>Unit</b> | <b>Value</b> | <b>Source</b>       | <b>Comment</b>                                                                                                                 |
| $\varepsilon^{\text{p}}$         | -           | 1.00         | —                   | pure nickel                                                                                                                    |

## 4 Initial Conditions

For the initial volume fractions of the evolving solid phases in the zinc electrode, i.e. especially for Zn and ZnO, see Table S3. Generally, volume fractions are locally set by using the tabulated value as a mean value plus a random noise (standard deviation of 1%). The volume fraction of the pore space is then adapted accordingly to fulfil locally the sum constraint  $\sum_{\alpha} \varepsilon^{\alpha} = 1$ , with  $\alpha$  being the locally occurring phases.

The electrolyte consists initially of a 7.4 M KOH solution, <sup>2</sup> which is saturated by ZnO (approx. 0.7 M). The maximum amount of ZnO which may be dissolved in a KOH solution varies with the KOH concentration, as it is depicted in Figure S3. <sup>9-13</sup> Regarding the experimental data given in the work of Takahashi, <sup>13</sup> the fit given by Kriegsmann and Cheh <sup>12</sup> matches the best and is used in this work:

$$c^{\text{sat, Zn(OH)}_4^{2-}} = -9.25 \cdot 10^{-5} + 0.0974c^{\text{K}^+} - 3.11 \left(c^{\text{K}^+}\right)^2 + 951 \left(c^{\text{K}^+}\right)^3 - 2.86 \cdot 10^4 \left(c^{\text{K}^+}\right)^4. \quad (2)$$

Note that the concentration  $c^{\text{K}^+}$  is in  $\text{mol cm}^{-3}$ , and the resulting saturation concentration is in  $\text{mol cm}^{-3}$ . A critical supersaturation, e.g. for nucleation of ZnO, is reached at  $c^{\text{crit, Zn(OH)}_4^{2-}} = 3.5c^{\text{sat, Zn(OH)}_4^{2-}}$ . <sup>4</sup> With this, the initial concentrations of the species  $\text{K}^+$ ,  $\text{OH}^-$  and  $\text{Zn(OH)}_4^{2-}$  may be calculated and are fixed.

**Table S4** Initial conditions in the electrolyte and the cathode material. Initial volume fractions may be found in Table S3

| <b>Electrolyte solution</b>     |                      |                      |                   |                                                                                                                                            |
|---------------------------------|----------------------|----------------------|-------------------|--------------------------------------------------------------------------------------------------------------------------------------------|
| Variable                        | Unit                 | Value                | Source            | Comment                                                                                                                                    |
| $c^{\text{K}^+}$                | $\text{mol cm}^{-3}$ | $7.4 \cdot 10^{-3}$  | Ref. <sup>2</sup> | —                                                                                                                                          |
| $c^{\text{OH}^-}$               | $\text{mol cm}^{-3}$ | $6.0 \cdot 10^{-3}$  | Ref. <sup>2</sup> | —                                                                                                                                          |
| $c^{\text{Zn(OH)}_4^{2-}}$      | $\text{mol cm}^{-3}$ | $0.7 \cdot 10^{-3}$  | Ref. <sup>2</sup> | —                                                                                                                                          |
| $c^{\text{O}_2(\text{aq})}$     | $\text{mol cm}^{-3}$ | $2.5 \cdot 10^{-8}$  | —                 | assumption: 10 % of the solubility in water at $T = 25^\circ\text{C}$ and $p = 1013.25\text{ hPa}$ , influence of electrolyte is neglected |
| $c^{\text{H}_2(\text{aq})}$     | $\text{mol cm}^{-3}$ | $4.3 \cdot 10^{-14}$ | —                 | assumption: 10 % of the solubility in water at $T = 25^\circ\text{C}$ and $p = 1013.25\text{ hPa}$ , influence of electrolyte is neglected |
| <b>Cathode active particles</b> |                      |                      |                   |                                                                                                                                            |
| Variable                        | Unit                 | Value                | Source            | Comment                                                                                                                                    |
| $c^{\text{H}^+}$                | $\text{mol cm}^{-3}$ | $4.4 \cdot 10^{-3}$  | —                 | from theoretic calculation; assuming an initial SOC of 0.5 %                                                                               |

## 5 Boundary Conditions

**Concentrations in the electrolyte solution** All concentration fields have a no flux (Neumann) boundary condition, i.e. the concentration flux  $\vec{N}^k|_{\partial V} = 0$  with  $k = \{\text{OH}^-, \text{Zn(OH)}_4^{2-}, \text{O}_2(\text{aq}), \text{H}_2(\text{aq})\}$ . Boundaries in y- and z-direction (not the thickness direction) may also be modelled as being periodic depending on the simulation setup. At internal boundaries, i.e. electrolyte/electrode interfaces, the respective reaction equations describe the production/consumption of specific species.

**Electric potential of the liquid phase** The electric potential of the liquid phase,  $\phi^l$ , has a no flux (Neumann) boundary condition stating the the ionic current  $\vec{j}^{\text{el}, l}|_{\partial V} = 0$ . Boundaries in y- and z-direction (not the thickness direction) may also be modelled as being periodic depending on the simulation setup. At internal electrolyte/electrode interfaces, the charge exchange influencing the electric potential of the solid phase is given by the respective reaction equations.

**Proton insertion into cathode active particles** The proton insertion and solid diffusion in active particles of the Ni cathode is modelled by a 1D model in spherical coordinates. The corresponding variable is the concentration of protons in the particle,  $c^{\text{H}^+}$ . At the particle surface there is a flux (Neumann) boundary condition which is proportional to the involved Butler-Volmer equation ( $\vec{N}^{\text{H}^+}|_{r=r_{\text{max}}} \propto \vec{j}^{\text{BV}}$ ), corrected by the respective specific and particle surface area and the number of particles, while the centre of the particle imposes a no flux (Neumann) boundary condition ( $\vec{N}^{\text{H}^+}|_{r=0} = 0$ ).

**Electric potential of the solid phase** The electric potential of the solid phase,  $\phi^s$  is the variable influenced by the applied cycling protocol. All surfaces are either no flux (Neumann) boundary condition ( $\vec{j}^{\text{el}, s}|_{\partial V} = 0$ ) or periodic boundary conditions (y- or z-direction depending on the setup), except the area defined as tab connection. In the pseudo-1D setup (see Figure S2a), the left and right boundaries

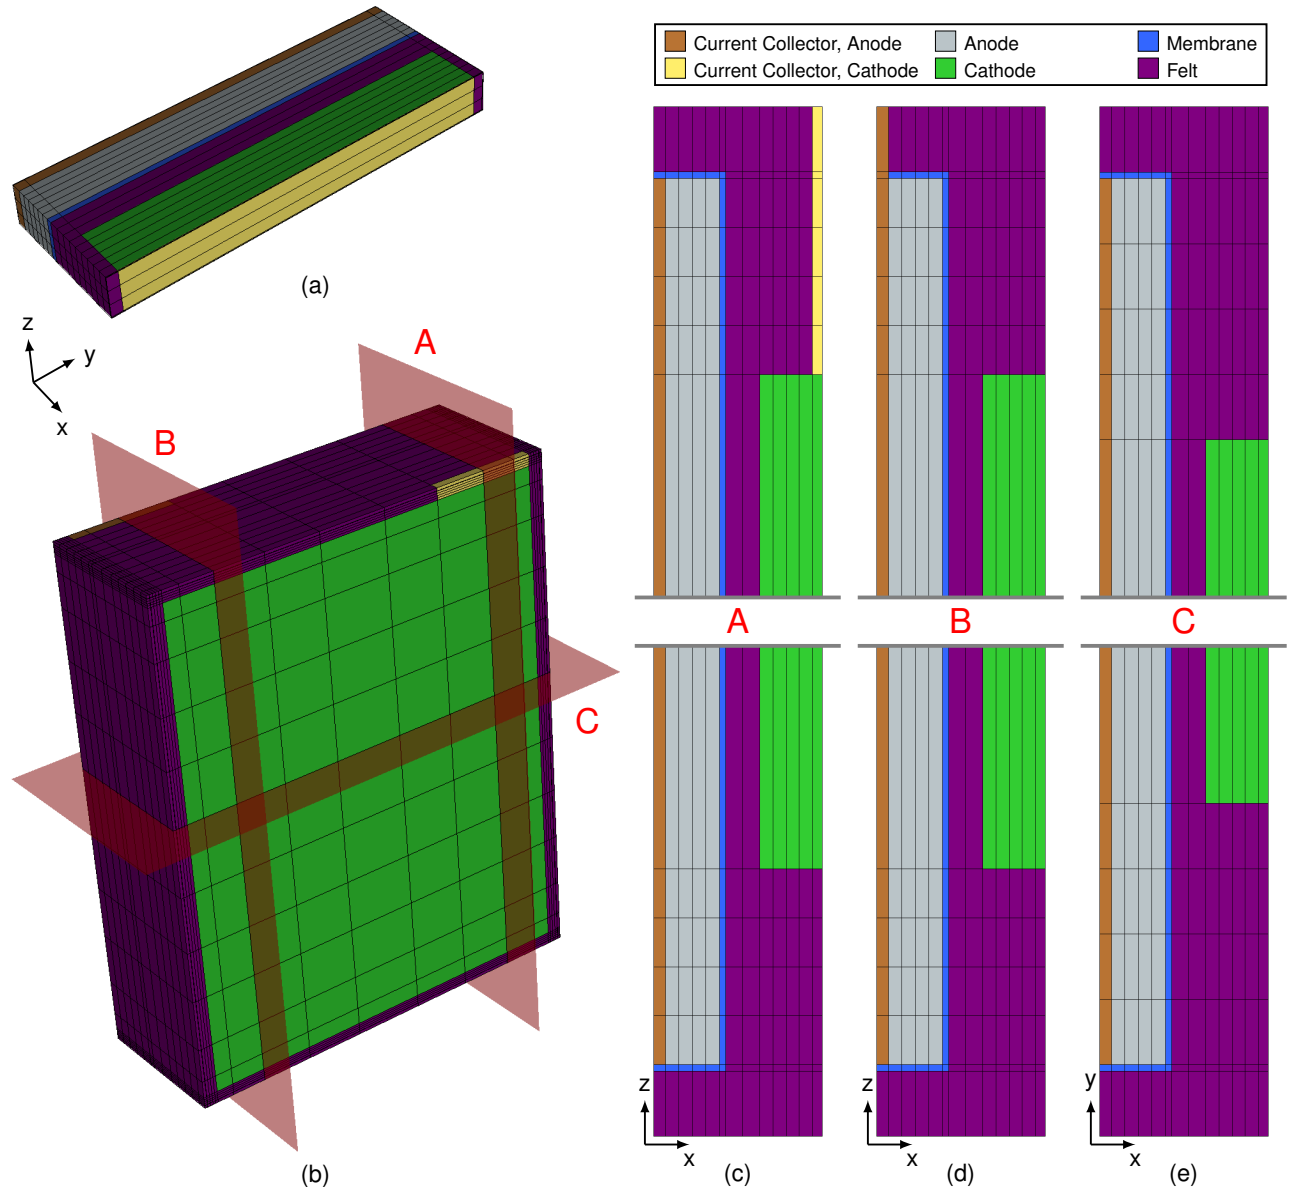

**Figure S2** Meshes and details on the simulation domains. (a) pseudo-1D domain (x-axis scaled by 20, z-axis by 5), (b) 3D domain (x-axis scaled by 20) with indicated cross-sectional cuts A, B and C, (c) vertical cut A through the Ni electrode tab connection, (d) vertical cut B through the Zn electrode tab connection, (e) horizontal cut C through the centre of the cell. The cuts focus on the outer regions of the cut direction.

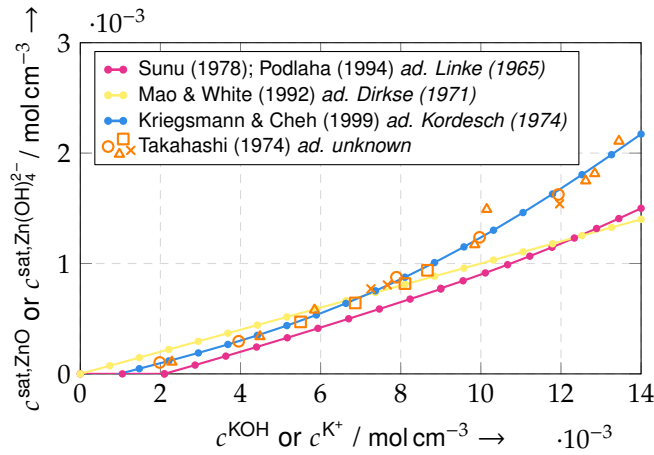

**Figure S3** Experimental data on saturation limits of  $\text{ZnO}/\text{Zn}(\text{OH})_4^{2-}$  in KOH solution from literature, and different fits found in literature.

( $x = 0$  and  $x = x^{\max}$ ) areas adjacent to the current collectors are the tabs of the electrochemical cell, in the 3D setup case (see Figure S2b), the top area of the small stripes leading to  $z = z^{\max}$  are the respective tabs of the anode and cathode. In both cases, a reference voltage is applied at the anode tab (Dirichlet boundary condition), while the cathode tab is used to apply boundary conditions in the sense of the cycling protocol, which may be a sequence of Dirichlet and/or Neumann boundary conditions (see below).

*Anode tab:*  $\phi^s = 0 \text{ V}$

*Cathode tab:* Here the charge and discharge conditions are applied (adapted from<sup>3</sup>).

- Formation cycles
  1. slow CC charge to full theoretical capacity
  2. slow CC discharge until  $U^{\text{cell}} < 1.2 \text{ V}$
  3. repeat
- Regular cycles (standard)
  1. CC charge with 1C until  $U^{\text{cell}} = 1.94 \text{ V}$
  2. CV charge with  $U^{\text{cell}} = 1.94 \text{ V}$  until transferred charge reaches 8 Ah
  3. CC discharge with 1C until  $U^{\text{cell}} < 1.0 \text{ V}$
  4. repeat
- Regular cycles (ZSW shape change experiment)
  1. CC charge with  $1/3\text{C}$  until transferred charge reaches 8 Ah
  2. CC discharge with 1C until  $U^{\text{cell}} < 1.0 \text{ V}$
  3. repeat

## 6 Solid Phases: Balance Equations and Material Parameters

### 6.1 Balance Equations

In the solid phase, two transport processes take place. Firstly, in solid regions throughout the cell charge conservation is enforced,

$$0 = -\vec{\nabla} \cdot (\vec{j}^{\text{el},s,\text{eff}}) + \sum_r A^r F z^r j^r \quad (3)$$

with:  $\vec{j}^{\text{el},s,\text{eff}} = -\frac{\epsilon^s}{\tau^s} \kappa^s \vec{\nabla} \phi^s$ ,

where  $\vec{j}^{\text{el},s,\text{eff}}$  is the effective electric current in the solid phase and the source term sum goes over all reactions  $r$ , with the appropriate specific surface  $A^r$ , charge number  $z^r$  and reaction rate  $j^r$ .  $F$  is the Faraday constant. The effective electric current is defined by Ohm's law, combining the gradient of the electric potential  $\phi^s$  in the solid phase with the conductivity  $\kappa^s$ . In the volume-averaged approach,  $\kappa^s$  has to be modified by the combined volume fraction of the solid phases,  $\epsilon^s$ , and the respective tortuosity  $\tau^s$  to account for the local microstructure. The total conductivity  $\kappa^s$  itself is calculated as an average value on the basis of the locally present solid phases and their conductivities (cf. Table S5).

The Zn electrode is a conversion electrode, i.e. Zn is dissolved and re-deposited during one discharge/charge cycle (cf. Zn dissolution reaction in Section section 9). Additionally, precipitation and dissolution of ZnO may take place (cf. ZnO precipitation reaction in Section section 9). This strong influence on the volume fractions in the Zn electrode has to be accounted for by appropriate balance equations,

$$\frac{\partial \varepsilon^\alpha}{\partial t} = \bar{V}^\alpha \sum_r A^r v^{\alpha r} j^r, \quad (4)$$

with  $\alpha = \{\text{Zn}, \text{ZnO}\}$ ,  $\bar{V}^\alpha$  the respective molar volume and  $v^{\alpha r}$  the stoichiometric coefficient of phase  $\alpha$  in reaction  $r$ .

A balance equation which is only solved in the Ni electrode concerns the insertion process of protons in the particles of the active material. This is modelled as spherical solid diffusion in radial direction,

$$\frac{\partial c^{\text{H}^+}}{\partial t} = \frac{1}{r^2} \frac{\partial}{\partial r} \left( D^{\text{H}^+} r^2 \frac{\partial c^{\text{H}^+}}{\partial r} \right), \quad (5)$$

where  $D^{\text{H}^+}$  is the diffusion coefficient of the protons in the NiO(OH)/Ni(OH)<sub>2</sub> particle.

## 6.2 Material Parameters

The conductivity of ZnO is calculated via the formula  $\kappa^{\text{ZnO}} = 0.01 \exp(-0.02/k_{\text{B}}T)$  (in  $\text{S cm}^{-1}$ ,  $T < 295.15 \text{ K}$  and  $k_{\text{B}}$  in  $\text{eV K}^{-1}$ ).<sup>14</sup> For the conductivity of the passive phase in the Zn anode, the conductivities of the single components (TiN<sup>15</sup>, Bi<sub>2</sub>O<sub>3</sub><sup>16</sup>, Ca(OH)<sub>2</sub><sup>17</sup> and PTFE<sup>18</sup>) have been used to calculate a Voigt average based on the presumed volume fractions. For the active material in the positive electrode, the conductivity depends on the state of charge (SOC) and is expressed as<sup>19, Eq. 20</sup>

$$\kappa^{\text{ca}}(\text{SOC}) = 0.1185 \exp(-8.459(1 - \text{SOC})^4). \quad (6)$$

Similarly, the proton diffusion parameter  $D^{\text{H}^+}$  in this material is as well SOC-dependent and follows<sup>20, Eq. 13</sup>

$$D^{\text{H}^+}(\text{SOC}) = D^{\text{H}^+, \text{NiO(OH)}} \left( \text{SOC} + \sqrt{D^{\text{H}^+, \text{NiO(OH)}}/D^{\text{H}^+, \text{Ni(OH)}_2}} (1 - \text{SOC}) \right)^2. \quad (7)$$

**Table S5** Material parameters of the solid phases

| Current collector anode           |                                |                       |                            |                                                                                                                                                     |
|-----------------------------------|--------------------------------|-----------------------|----------------------------|-----------------------------------------------------------------------------------------------------------------------------------------------------|
| Variable                          | Unit                           | Value                 | Source                     | Comment                                                                                                                                             |
| $\kappa^{\text{Cu}}$              | $\text{S cm}^{-1}$             | $5.96 \cdot 10^5$     | Ref. <sup>21</sup>         | pure copper ( $T = 20^\circ \text{C}$ )                                                                                                             |
| Anode                             |                                |                       |                            |                                                                                                                                                     |
| Variable                          | Unit                           | Value                 | Source                     | Comment                                                                                                                                             |
| $\kappa^{\text{P}}$               | $\text{S cm}^{-1}$             | $5.328 \cdot 10^3$    | —                          | mixture of TiN <sup>15</sup> , Bi <sub>2</sub> O <sub>3</sub> <sup>16</sup> , Ca(OH) <sub>2</sub> <sup>17</sup> and PTFE <sup>18</sup> (approx. RT) |
| $\kappa^{\text{Zn}}$              | $\text{S cm}^{-1}$             | $1.689 \cdot 10^5$    | Ref. <sup>22</sup>         | for $T = 295 \text{ K}$                                                                                                                             |
| $\kappa^{\text{ZnO}}$             | $\text{S cm}^{-1}$             | $4.555 \cdot 10^{-3}$ | Ref. <sup>14</sup>         | formula evaluated for $T = 25^\circ \text{C}$                                                                                                       |
| $\bar{V}^{\text{Zn}}$             | $\text{cm}^3 \text{ mol}^{-1}$ | 9.161                 | —                          | —                                                                                                                                                   |
| $\bar{V}^{\text{ZnO}}$            | $\text{cm}^3 \text{ mol}^{-1}$ | 14.508                | —                          | —                                                                                                                                                   |
| Membrane                          |                                |                       |                            |                                                                                                                                                     |
| Variable                          | Unit                           | Value                 | Source                     | Comment                                                                                                                                             |
| $\kappa^{\text{P}}$               | $\text{S cm}^{-1}$             | 0.0                   | —                          | assumption: no electric conduction                                                                                                                  |
| Felt                              |                                |                       |                            |                                                                                                                                                     |
| Variable                          | Unit                           | Value                 | Source                     | Comment                                                                                                                                             |
| $\kappa^{\text{P}}$               | $\text{S cm}^{-1}$             | 0.0                   | —                          | assumption: no electric conduction                                                                                                                  |
| Cathode                           |                                |                       |                            |                                                                                                                                                     |
| Variable                          | Unit                           | Value                 | Source                     | Comment                                                                                                                                             |
| $\kappa^{\text{P}}$               | $\text{S cm}^{-1}$             | $1.429 \cdot 10^5$    | Ref. <sup>22</sup>         | assumption: mostly a nickel mesh; hence pure nickel ( $T = 295 \text{ K}$ )                                                                         |
| $\kappa^{\text{ca}}$              | $\text{S cm}^{-1}$             | (6)                   | Ref. <sup>19, Eq. 20</sup> | dependent on state of charge (SOC)                                                                                                                  |
| $D^{\text{H}^+}$                  | $\text{cm}^2 \text{ s}^{-1}$   | (7)                   | Ref. <sup>20, Eq. 13</sup> | dependent on state of charge (SOC)                                                                                                                  |
| $D^{\text{H}^+, \text{Ni(OH)}_2}$ | $\text{cm}^2 \text{ s}^{-1}$   | $1.0 \cdot 10^{-12}$  | —                          | fitting parameter; inspired by Ref. <sup>20</sup> , range of values reported in Ref. <sup>19</sup>                                                  |
| $D^{\text{H}^+, \text{NiO(OH)}}$  | $\text{cm}^2 \text{ s}^{-1}$   | $9.5 \cdot 10^{-11}$  | —                          | fitting parameter; inspired by Ref. <sup>20</sup> , range of values reported in Ref. <sup>19</sup>                                                  |
| Current collector cathode         |                                |                       |                            |                                                                                                                                                     |
| Variable                          | Unit                           | Value                 | Source                     | Comment                                                                                                                                             |
| $\kappa^{\text{Ni}}$              | $\text{S cm}^{-1}$             | $1.429 \cdot 10^5$    | Ref. <sup>22</sup>         | pure nickel ( $T = 295 \text{ K}$ )                                                                                                                 |



## 7 Liquid Phase: Balance Equations and Material Parameters

The model equations for the convection of the electrolyte solution are not discussed here, but in the separate section 11.

### 7.1 Balance Equations

The transport of charged particles in the electrolyte solution is one of the core elements of a battery model. As in the solid phases (see section 6), a volume-averaged approach is chosen here and additionally concentrated solution theory applies due to the highly concentrated alkaline electrolyte solution (see Table S4).

For the charged particles, the ions  $k = \{\text{OH}^-, \text{Zn}(\text{OH})_4^{2-}\}$ , transport comprises diffusion, electromigration and convection and is written as

$$\begin{aligned} \frac{\partial \varepsilon^1 c^k}{\partial t} &= -\vec{\nabla} \cdot (\vec{N}^{k,\text{eff}} + \varepsilon^1 c^k \vec{v}) + \sum_r A^r v^{kr} j^r \\ \text{with: } \vec{N}^{k,\text{eff}} &= -\frac{\varepsilon^1}{\tau^1} D^k \vec{\nabla} c^k + \frac{t^k}{z^k F} \vec{j}^{\text{el},1,\text{eff}}, \end{aligned} \quad (8)$$

with  $\vec{N}^{k,\text{eff}}$  being the effective concentration flux density,  $\vec{v}$  the volume-centred convection velocity,<sup>23,24</sup> and the source term as previously (e.g. Equation 4). Species transport and charge conservation are strongly coupled in the electrolyte solution, which reflects when  $\vec{N}^{k,\text{eff}}$  is looked at: The first term represents diffusion with the diffusion coefficient  $D^k$  and the concentration gradient  $\vec{\nabla} c^k$ , which are corrected by  $\varepsilon^1/\tau^1$  to account for the microstructure. The second term is the coupling with the electrolyte potential, represented by the effective ionic current density  $\vec{j}^{\text{el},1,\text{eff}}$ , of which the fraction  $t^k$  drives the transport of charged species  $k$ . This is the transference number, which follows a sum constraint over all charged particles in solution,  $\sum_k t^k = 1$  for  $k = \{\text{K}^+, \text{OH}^-, \text{Zn}(\text{OH})_4^{2-}\}$ .

This strong coupling is mirrored in the charge conservation, which writes analogously to Equation 3 as

$$\begin{aligned} 0 &= -\vec{\nabla} \cdot (\vec{j}^{\text{el},1,\text{eff}}) + \sum_r A^r F z^r j^r \\ \text{with: } \vec{j}^{\text{el},1,\text{eff}} &= -\frac{\varepsilon^1}{\tau^1} \kappa^1 \vec{\nabla} \phi^1 - \frac{\varepsilon^1}{\tau^1} \frac{\kappa^1}{F} \sum_k \frac{t^k}{z^k} \left( \frac{\partial \mu^k}{\partial c^k} \right) \vec{\nabla} c^k. \end{aligned} \quad (9)$$

The effective ionic current density consists as well of two parts: The first part is an analogon to Ohm's law in solids with the ionic conductivity of the electrolyte solution,  $\kappa^1$ , and the gradient of the electric potential in the electrolyte solution,  $\vec{\nabla} \phi^1$ . The second part gives the fraction of ionic current density induced by diffusion of charged species. Here, the thermodynamic factor  $(\partial \mu^k / \partial c^k)$  with chemical potential  $\mu^k = \mu^{k,\circ} + RT \ln a^k$  has to be mentioned, where, when derived by  $c^k$ , we tacitly assume that the activity coefficient in  $a^k = \gamma^k c^k$  is constant. Likewise, the standard chemical potential of species  $k$ ,  $\mu^{k,\circ}$ , is constant.

For the uncharged gas molecules dissolved in the electrolyte solution,  $k = \{\text{O}_2(\text{aq}), \text{H}_2(\text{aq})\}$ , a transport law similar to Equation 8 is used,

$$\begin{aligned} \frac{\partial \varepsilon^1 c^k}{\partial t} &= -\vec{\nabla} \cdot (\vec{N}^{k,\text{eff}} + \varepsilon^1 c^k \vec{v}) + \sum_r A^r v^{kr} j^r \\ \text{with: } \vec{N}^{k,\text{eff}} &= -\frac{\varepsilon^1}{\tau^1} D^k \vec{\nabla} c^k. \end{aligned} \quad (10)$$

Here only diffusion and convection plays a role.

Lastly, at the Zn electrode, two surface concentrations are calculated. These arise due to the fact that a ZnO passivation layer may form around Zn particles (cf. ZnO precipitation reaction in Section section 9), which hinders the species transport to the Zn particle surface affecting Zn dissolution and H<sub>2</sub> formation reactions. The balance equation reads

$$\left(1 - \varepsilon^{\text{ZnO-L}}\right) \beta^{\text{ZnO-L}} D^k \frac{r^{\text{ZnO,o}}}{r^{\text{ZnO,i}}} \frac{(c^{k,s} - c^k)}{\Delta^{\text{ZnO}}} = \sum_r v^{kr} j^r, \quad (11)$$

which is the volume-averaged concentration flux density due to diffusion through the ZnO layer in balance with the relevant reactions on the Zn particle surface. While the source term on the right-hand side has its usual meaning, the left-hand side resembles a radial diffusion term. The solid phase volume fraction  $\varepsilon^{\text{ZnO-L}}$  and the Bruggeman coefficient  $\beta^{\text{ZnO-L}}$  modify the diffusion coefficient  $D^k$  to an effective parameter, and the remaining part is the concentration gradient through the ZnO layer consisting of the surface concentration  $c^{k,s}$ , the usual bulk concentration  $c^k$ , the thickness of the ZnO layer  $\Delta^{\text{ZnO}}$  and the respective outer and inner radii,  $r^{\text{ZnO,o}}$  and  $r^{\text{ZnO,i}}$ .

### 7.2 Material Parameters

Following the derivation of the model presented in Latz and Zausch,<sup>25</sup> or similar work such as Katchalsky and Curran<sup>26</sup> or Fong *et al.*,<sup>27</sup> the diffusion coefficients  $D^k$  of the species  $\text{OH}^-$  and  $\text{Zn}(\text{OH})_4^{2-}$  is characterised by their respective salt/electrolyte (i.e. KOH and  $\text{K}_2\text{Zn}(\text{OH})_4$ ), and with respect to the electrolyte solution as a whole. The transference numbers  $t^k$  however are a parameter unique to each ion (i.e.  $\text{OH}^-$ ,  $\text{Zn}(\text{OH})_4^{2-}$  and  $\text{K}^+$ ). The remaining transport parameter, the ionic conductivity  $\kappa^1$ , is linked to the electrolyte solution in total, i.e. with respect to all dissolved species. Generally, due to the highly concentrated electrolyte, no dilute solution equations can be used to estimate transport parameters. Here we rely solely on experimental findings and trends.

Besides the transport parameters intrinsic to the electrolyte chosen, we list here as well the diffusion coefficients of the dissolved gases O<sub>2</sub> and H<sub>2</sub>.

**Diffusion coefficients** For the diffusion coefficient of the hydroxide ions, i.e.  $D^{\text{KOH}}$ , we choose the function as fitted by Paxton and Newman<sup>28</sup> based on the experiments of Bhatia *et al.*<sup>29</sup> (see Figure S4). This is given by

$$D^{\text{KOH}} = 2.8509 \cdot 10^{-5} - 2.9659 \cdot 10^{-4} \sqrt{c^{\text{K}^+}} + 0.013768 c^{\text{K}^+} - 0.14199 \left(c^{\text{K}^+}\right)^{\frac{3}{2}} + 0.42661 \left(c^{\text{K}^+}\right)^2 \text{ in cm}^2 \text{ s}^{-1}, \quad (12)$$

where  $c^{\text{K}^+}$  is the concentration of potassium ions in  $\text{mol cm}^{-3}$ . Here we assumed that  $D^{\text{KOH}}$  is largely independent of the zincate concentration, and hence the  $\text{K}^+$  concentration should be the relevant quantity to determine this diffusion coefficient. Following May and

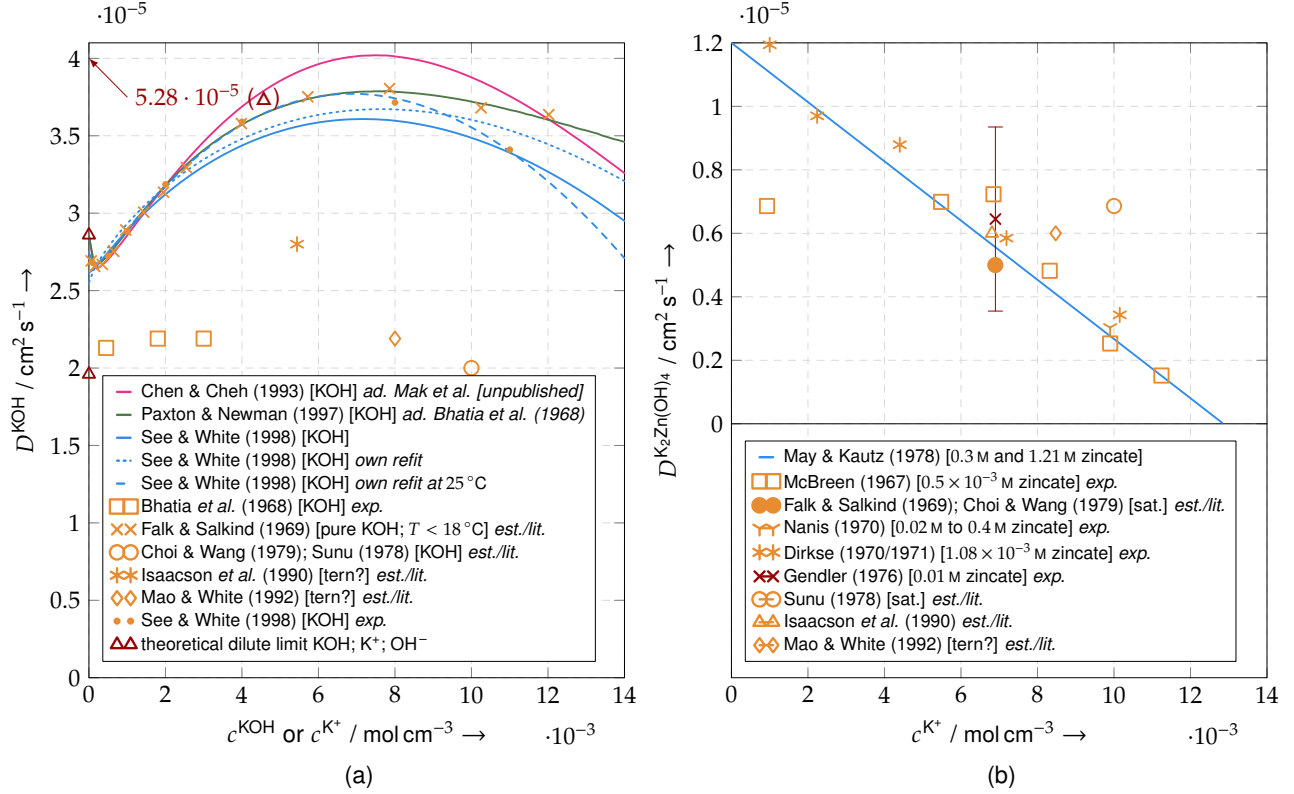

**Figure S4** Selection of experimental<sup>29–34</sup> and estimated<sup>9,11,35–37</sup> diffusion coefficients for KOH and  $\text{K}_2\text{Zn}(\text{OH})_4$  from literature, and some associated fits.<sup>28,30,38,39</sup> The fit done by See and White<sup>30</sup> seems to be not correctly stated in their work, as it fits only poorly their experimental results. For this reason, two re-fits were performed (with and without temperature dependence).

Kautz,<sup>39</sup> the diffusion coefficient of the zincate ion, i.e.  $D^{\text{K}_2\text{Zn}(\text{OH})_4}$ , is modelled concentration-dependent as

$$D^{\text{K}_2\text{Zn}(\text{OH})_4} = 12.00 \cdot 10^{-6} - 9.33 \cdot 10^{-4} \cdot c^{\text{K}^+} \text{ in cm}^2 \text{ s}^{-1}, \quad (13)$$

where  $c^{\text{K}^+}$  is the concentration of potassium ions in  $\text{mol cm}^{-3}$ .

**Electrolyte conductivity** From literature (cf. Figure S5a) a strong dependence of the electrolyte conductivity  $\kappa^1$  on the KOH concentration in the electrolyte solution is known. When adding and saturating the solution with ZnO, the produced  $\text{Zn}(\text{OH})_4^{2-}$  diminishes  $\kappa^1$  in a linear manner<sup>40–42</sup>. The y-intercept is the ionic conductivity for the pure KOH solution, and the slope is dependent on this KOH concentration. It has been observed, that higher initial KOH concentrations produce flatter slopes, as the ratio of  $\text{Zn}(\text{OH})_4^{2-}$  to  $\text{OH}^-$  is smaller (see Figure S5b). Liu *et al.*<sup>41</sup> give for initial KOH concentrations in the range of 6.9 M to 7.4 M at around room temperature the relation  $\kappa = (0.637 \pm 0.011) - (0.159 \pm 0.009) c^{\text{Zn}(\text{OH})_4^{2-}} / c^\circ$ .

Here we assume, that the magnitude of the initial conductivity and this slope is approximately also valid for our initial KOH concentration of 7.4 M. From this we construct a function dependent on  $c^{\text{K}^+}$  and  $c^{\text{Zn}(\text{OH})_4^{2-}}$ , using the fits of Paxton and Newman<sup>28</sup> and Liu *et al.*<sup>41</sup>:

$$\kappa^1 = \kappa^{\text{Paxton}} - 0.159 \frac{c^{\text{Zn}(\text{OH})_4^{2-}}}{c^\circ} \text{ in S cm}^{-1} \quad (14)$$

$$\text{with } \kappa^{\text{Paxton}} = 0.02325 + 210.95 c^{\text{K}^+} - 22077 \left(c^{\text{K}^+}\right)^2 + 6.2907 \cdot 10^5 \left(c^{\text{K}^+}\right)^3,$$

where  $\kappa^{\text{Paxton}}$  is the conductivity without any zincate present. As the local  $\text{K}^+$  concentration (in  $\text{mol cm}^{-3}$ ) is not expected to vary too much in our simulations, we assume that the slope due to zincate addition stays constant at 0.159. Equation 14 is depicted in Figure S5c.

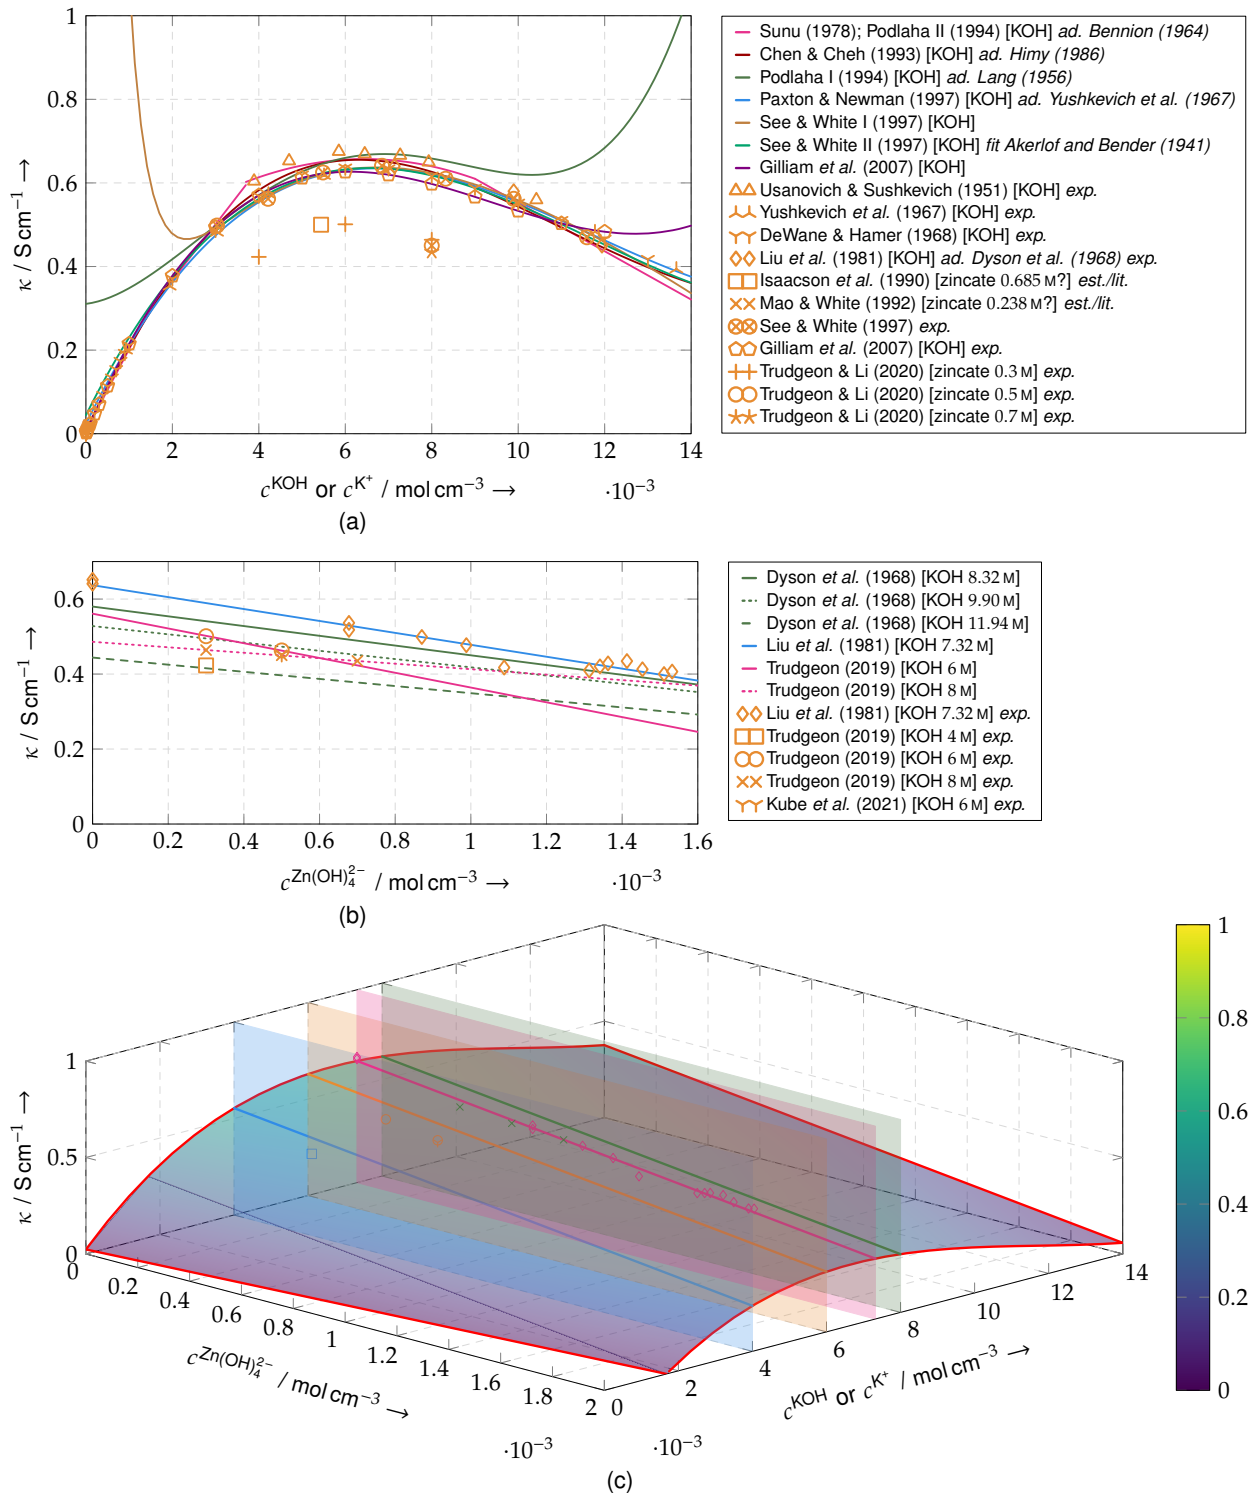

**Figure S5** Electrolyte conductivity  $\kappa^l$  depicted due to the dependence on (a) the KOH/ $\text{K}^+$  concentration in a pure KOH electrolyte solution and (b) the  $\text{Zn(OH)}_4^{2-}$  concentration in a KOH- $\text{K}_2\text{Zn(OH)}_4$  electrolyte solution. Experimental<sup>41–53</sup> and estimated<sup>11,37</sup> data as well as fits<sup>9,10,28,38,40–42,47,48</sup> are taken from literature. In (c) a simple function for  $\kappa^l$  dependent on both concentrations is shown, which is used in the simulations.

**Transference numbers** To calculate the transference numbers of the species contained in the electrolyte solution we follow three basic assumptions:

- Following Lengyel *et al.*,<sup>54</sup>  $t^{K^+} = 0.22$  within  $c^{KOH} = 3\text{ M}$  to  $12\text{ M}$ . We assume that this holds as well for a  $KOH\text{-}K_2Zn(OH)_4$  electrolyte solution, and that the ratio of the anions ( $OH^-$  to  $Zn(OH)_4^{2-}$ ) within the solubility limit (Equation (2)) does not affect this value.
- Due to the sum constraint  $\sum_i t^i = 1$ ,  $t^{OH^-}$  may be calculated by using the other two transference numbers.
- The only transference number to be explicitly calculated is  $t^{Zn(OH)_4^{2-}}$ . As the solubility limit in the relevant  $KOH$  concentration range is mostly  $c^{Zn(OH)_4^{2-}} < 1\text{ M}$ , it is deemed acceptable to use dilute solution theory for this calculation.

A definition for the transference number not limited to dilute solution theory is  $t^k = \kappa^k / \kappa^l$ , which uses the ratio of the ionic conductivity of species  $k$  to the total ionic conductivity of the electrolyte solution. Using dilute solution theory,  $\kappa^{Zn(OH)_4^{2-}}$  may be calculated via

$$\kappa^{Zn(OH)_4^{2-}} = \left( z^{Zn(OH)_4^{2-}} \right)^2 c^{Zn(OH)_4^{2-}} D^{Zn(OH)_4^{2-}} \frac{F^2}{RT}, \quad (15)$$

where  $z^{Zn(OH)_4^{2-}} = -2$  is the charge number of zincate, and  $c^{Zn(OH)_4^{2-}}$  and  $D^{Zn(OH)_4^{2-}}$  are its concentration and diffusion coefficient, respectively. It has to be noted, that  $D^{Zn(OH)_4^{2-}} \neq D^{K_2Zn(OH)_4}$  introduced in Equation 13. This unknown diffusion coefficient is calculated using another dilute solution relation,<sup>55</sup>

$$D^{K_2Zn(OH)_4} = \frac{D^{K^+} D^{Zn(OH)_4^{2-}} \left( \left( z^{K^+} \right)^2 c^{K^+} + \left( z^{Zn(OH)_4^{2-}} \right)^2 c^{Zn(OH)_4^{2-}} \right)}{\left( z^{K^+} \right)^2 c^{K^+} D^{K^+} + \left( z^{Zn(OH)_4^{2-}} \right)^2 c^{Zn(OH)_4^{2-}} D^{Zn(OH)_4^{2-}}}, \quad (16)$$

which has to be solved for  $D^{Zn(OH)_4^{2-}}$ . Here we have additionally the charge number of potassium,  $z^{K^+} = +1$ , its concentration  $c^{K^+}$  in  $K_2Zn(OH)_4$  and its dilute limit diffusion coefficient  $D^{K^+} = 1.957 \cdot 10^{-5} \text{ cm}^2 \text{ s}^{-1}$  (see e.g. Newman and Balsara<sup>56</sup>). The diffusion coefficient  $D^{K_2Zn(OH)_4}$  is calculated using the previously stated Equation 13. Regarding the concentrations used in this equation care has to be taken:

- to calculate  $D^{K_2Zn(OH)_4}$ , Equation 13, the usual  $c^{K^+} = c^{OH^-} + 2c^{Zn(OH)_4^{2-}}$  has to be taken
- the concentrations  $c^{K^+}$  and  $c^{Zn(OH)_4^{2-}}$  mentioned in Equation (16) are taken as the maximum possible, i.e.  $c^{Zn(OH)_4^{2-}} = c^{\text{sat}, Zn(OH)_4^{2-}}$  (see Equation 2) and stemming from this  $c^{K^+} = 2c^{\text{sat}, Zn(OH)_4^{2-}}$  to satisfy the composition of  $K_2Zn(OH)_4$ .

The resulting  $t^{Zn(OH)_4^{2-}}$  rises nearly linearly with increasing  $c^{Zn(OH)_4^{2-}}$ , with  $t^{Zn(OH)_4^{2-}} = 0$  for  $c^{Zn(OH)_4^{2-}} = 0$  and goes up to about  $t^{Zn(OH)_4^{2-}} \approx 0.1$  around the saturation limit. Accordingly,  $t^{OH^-} = 1.0 - t^{K^+} - t^{Zn(OH)_4^{2-}}$  drops with increasing  $c^{Zn(OH)_4^{2-}}$ .

**Transport of gases** The oxygen and hydrogen produced at the cathode and anode, respectively (cf. section 9), dissolves in the electrolyte solution and may hence diffuse within the liquid. Tham *et al.*<sup>57</sup> measured the respective diffusion coefficients for a pure  $KOH$  electrolyte solution, and Hodges *et al.*<sup>58</sup> provide a fit for the measured data (dependent on  $KOH$  concentration and temperature). We assume that these diffusion coefficients are only weakly dependent on the  $Zn(OH)_4^{2-}$  concentration, and therefore the utilisation of a pure  $KOH$  dependence is acceptable. Furthermore, as we operate our electrochemical cell at a constant temperature, we re-fitted the provided data for  $T = 25^\circ\text{C}$  and molar concentration. Using the same fitting functions, we state

$$D^{O_2(aq)} = 1.785 \cdot 10^{-5} - 3.505 \cdot 10^{-6} \frac{c^{K^+}}{c^o} + 3.183 \cdot 10^{-7} \left( \frac{c^{K^+}}{c^o} \right)^2 - 1.170 \cdot 10^{-8} \left( \frac{c^{K^+}}{c^o} \right)^3 + 1.015 \cdot 10^{-10} \left( \frac{c^{K^+}}{c^o} \right)^4 \text{ in } \text{cm}^2 \text{ s}^{-1}, \quad (17)$$

and

$$D^{H_2(aq)} = 3.466 \cdot 10^{-5} - 4.764 \cdot 10^{-6} \frac{c^{K^+}}{c^o} + 3.801 \cdot 10^{-7} \left( \frac{c^{K^+}}{c^o} \right)^2 - 1.125 \cdot 10^{-8} \left( \frac{c^{K^+}}{c^o} \right)^3 \text{ in } \text{cm}^2 \text{ s}^{-1}, \quad (18)$$

where  $c^{K^+}$  is the concentration of potassium ions in  $\text{mol cm}^{-3}$ .

**Table S6** Parameters of the electrolyte solution

| Diffusivities     |                              |       |            |                                       |
|-------------------|------------------------------|-------|------------|---------------------------------------|
| Variable          | Unit                         | Value | Source     | Comment                               |
| $D^{KOH}$         | $\text{cm}^2 \text{ s}^{-1}$ | (12)  | Ref. 28,29 | —                                     |
| $D^{K_2Zn(OH)_4}$ | $\text{cm}^2 \text{ s}^{-1}$ | (13)  | Ref. 39,59 | —                                     |
| $D^{O_2(aq)}$     | $\text{cm}^2 \text{ s}^{-1}$ | (17)  | Ref. 57,58 | own re-fit for $T = 25^\circ\text{C}$ |
| $D^{H_2(aq)}$     | $\text{cm}^2 \text{ s}^{-1}$ | (18)  | Ref. 57,58 | own re-fit for $T = 25^\circ\text{C}$ |
| Conductivities    |                              |       |            |                                       |
| Variable          | Unit                         | Value | Source     | Comment                               |

| $\kappa$                    | $\text{Scm}^{-1}$ | (14)                                                  | Ref. <sup>28,41</sup> | combined fits of Paxton and Newman <sup>28</sup> and Liu <i>et al.</i> <sup>41</sup>                     |
|-----------------------------|-------------------|-------------------------------------------------------|-----------------------|----------------------------------------------------------------------------------------------------------|
| <b>Transference Numbers</b> |                   |                                                       |                       |                                                                                                          |
| Variable                    | Unit              | Value                                                 | Source                | Comment                                                                                                  |
| $t^{K^+}$                   | —                 | 0.22                                                  | Ref. <sup>54</sup>    | assumed to be constant in relevant range of anion concentrations                                         |
| $t^{Zn(OH)_4^{2-}}$         | —                 | $t^k = \kappa^k / \kappa^l$<br>with Eq. (15) and (16) | —                     | as mostly $c^{Zn(OH)_4^{2-}} < 1 \text{ M}$ , we assume that dilute solution theory formulas may be used |
| $t^{OH^-}$                  | —                 | $1.0 - t^{K^+} - t^{Zn(OH)_4^{2-}}$                   | —                     | —                                                                                                        |

## 8 Gas Phase: Balance Equations and Material Parameters

The gas phase serves solely as a volume buffer for the convection model, which follows the sum constraint on volume fractions,  $\epsilon^g = 1 - \sum \alpha \epsilon^\alpha$  with  $\alpha$  being all locally present solid and liquid phases. A change in gas volume fraction does not affect the gas pressure, which always rests at  $p^g = p^{\text{atm}} = 1013.25 \text{ hPa} = \text{const.}$  (cf. section 11). Furthermore, the gas concentrations  $c^{\text{H}_2(g)}$  and  $c^{\text{O}_2(g)}$  resulting from the outgassing reactions are only stored in this phase, but neither have they any influence on the battery cell nor are they transported in any way.

## 9 Reactions and Reaction Parameters

In the following, all reactions used in our model are introduced and motivated. These are rooted in the concept of Doppl<sup>1</sup>, especially those concerning the Ni electrode and the gas balance. We restrict ourselves here to purely physico-chemical aspects. From a numerical point of view, some reaction rates may feature a variable pre-factor, which asymptotically slows down reactions when affected concentrations or volume fractions approach zero to maintain a stable simulation. This factor is not included in the following equations.

**Zinc dissolution (zinc electrode)** Reaction:

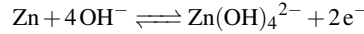

The zinc dissolution reaction is modelled by a Butler-Volmer reaction rate,

$$j^I = -k^I \left( \frac{c^{\text{Zn(OH)}_4^{2-}}}{c^\circ} \right)^{(1-\alpha^I)} \left( \frac{c^{\text{(OH)}^-}}{c^\circ} \right)^{4\alpha^I} \left\{ \left( \frac{c^{\text{Zn(OH)}_4^{2-},s}}{c^{\text{Zn(OH)}_4^{2-}}} \right) e^{-\alpha^I \frac{j_F}{RT} \eta^I} - \left( \frac{c^{\text{OH}^-,s}}{c^{\text{OH}^-}} \right)^4 e^{(1-\alpha^I) \frac{j_F}{RT} \eta^I} \right\}, \quad (19)$$

with the fitted reaction rate constant  $k^I = 2.50 \cdot 10^{-10} \text{ mol cm}^{-2} \text{ s}^{-1}$  and the overpotential  $\eta^I = \Delta\phi - \left\{ \Delta\phi^{\circ,I} + \frac{RT}{z^I F} \ln \left( \frac{c^{\text{Zn(OH)}_4^{2-}}}{c^\circ} / \left( \frac{c^{\text{OH}^-}}{c^\circ} \right)^4 \right) \right\}$ , with  $\Delta\phi^{\circ,I}$  being the standard reduction potential.

The form chosen here follows two considerations: Despite the multi-step character of this reaction,<sup>60</sup> we choose to model it as a one-step reaction with  $\alpha^I = 0.5$  and  $z^I = 2$  as it is unclear whether the same rate-determining step persists with our electrode composition and in our electrolyte environment. Furthermore, due to the ZnO layer around the Zn particle surface, we already include surface concentrations in our model. To use them consistently, we consider these mass-transfer effects in Butler-Volmer equation following e.g. Bard and Faulkner<sup>61</sup>, Eq. 3.4.10. Lastly, the standard reduction potential has been modified to  $\Delta\phi^{\circ,I} = -1.199 \text{ V} - 0.045 \text{ V} - 0.025 \text{ V} = -1.269 \text{ V/SHE}$ . While the first value is the literature value at standard conditions,<sup>62</sup> the second and third value are corrections due to the concentration overpotential. A first correction is made on basis of the activity coefficients<sup>63</sup>, Eq. 1 at the initial electrolyte solution composition (cf. Table S4), and a second one due to the assumption, that the  $\text{Ca(OH)}_2$  in the Zn electrode lowers the amount of dissolved zincate in the electrolyte,<sup>64</sup> an effect which is not included in the model presented here and hence artificially added in the standard reduction potential.

**Proton insertion (nickel electrode)** Reaction:

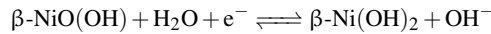

The proton insertion reaction is modelled by a one-step and symmetric ( $\alpha^{\text{II}} = 0.5$ ) Butler-Volmer reaction rate,

$$j^{\text{II}} = k^{\text{II}} \left( \text{SOC}^{\text{red.}} \right)^{(1-\alpha^{\text{II}})} \left( \text{SOC}^{\text{ox.}} \frac{c^{\text{(OH)}^-}}{c^\circ} \right)^{\alpha^{\text{II}}} \left\{ e^{-\alpha^{\text{II}} \frac{j_F}{RT} \eta^{\text{II}}} - e^{(1-\alpha^{\text{II}}) \frac{j_F}{RT} \eta^{\text{II}}} \right\}, \quad (20)$$

where  $k^{\text{II}} = 1 \cdot 10^{-7} \text{ mol cm}^{-2} \text{ s}^{-1}$  is the fitted reaction rate constant and  $\text{SOC}^{\text{ox.}} = 1 - \text{SOC}^{\text{red.}}$  is the state-of-charge regarding the oxidised and reduced state, with  $\text{SOC}^{\text{red.}} = c^{\text{H}^+} / c^{\text{H}^+, \text{max}}$ . The charge number is  $z^{\text{II}} = 1$  and the overpotential  $\eta^{\text{II}} = \Delta\phi - \left\{ \Delta\phi^{\circ,\text{II}}(\text{SOC}^{\text{red.}}) + \frac{RT}{z^{\text{II}} F} \ln \left( c^\circ / c^{\text{OH}^-} \right) \right\}$ .

The OCV curve,  $\Delta\phi^{\circ,\text{II}}(\text{SOC}^{\text{red.}})$ , is based on Malaie *et al.* <sup>65</sup>, Eq. 17 (or see Watanabe and Kumagai<sup>66,67</sup> for a more experimental approach), but without using their term for a phase transformation. This is the behaviour of a binary real solution, where particle interactions  $A-A$ ,  $B-B$  and  $A-B$  may be all different. Unlike Malaie *et al.* <sup>65</sup>, we state that our solvent is  $\text{NiO(OH)}$  ( $A$ ) and our solute is  $\text{H}^+$  ( $B$ ); which resembles the amount of  $\text{Ni(OH)}_2$ . Having this perception, we may argue that the  $A-B$  interaction is favourable

as we have insertion of  $H^+$  into  $NiO(OH)$ , and hence we must set their interaction parameter  $2g = \gamma < 0$  and choose the limit case  $2g = \gamma = -8$ .<sup>68, Sec. 5.4</sup> The equation reads then

$$\Delta\phi^{\circ,II}(\text{SOC}^{\text{red.}}) = \Delta\phi^{\circ,II} + \Delta\phi^{\text{hyst.}} + \frac{RT}{z_{II}F} \left( \ln \left( \frac{\text{SOC}^{\text{ox.}}}{\text{SOC}^{\text{red.}}} \right) - \frac{1}{4} \gamma (1 - 2 \cdot \text{SOC}^{\text{red.}}) \right) \quad (21)$$

and is shown in Figure S6. The standard reduction potential, which is given for this reaction type at 50 % discharge, i.e. the reduction direction, is similarly modified as it is done for the Zn dissolution reaction. We assume  $\Delta\phi^{\circ,II} = 0.49 \text{ V} - 0.045 \text{ V} - 0.08 \text{ V} = 0.365 \text{ V/SHE}$ , consisting of the literature value at standard conditions,<sup>62</sup> the influence of the activity coefficients<sup>63, Eq. 1</sup> at the initial conditions of the cell (cf. Table S4) and a modification due to Co additives and other influences. Furthermore, the Ni electrode shows a charge/discharge hysteresis, which varies with e.g. electrode composition and additives,<sup>19,69–71</sup> and whose true origin is still disputed. Due to the unclear physical basis, we model this hysteresis as a simple offset by  $\Delta\phi^{\text{hyst.}} = 132.5 \text{ mV}$  when charging the electrochemical cell.

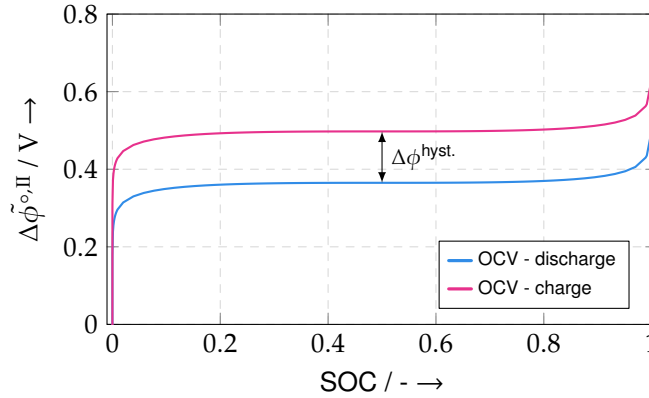

**Figure S6** The charge and discharge branch of the OCV depended on the SOC. To mimic a hysteresis, the charge branch is shifted by  $\Delta\phi^{\text{hyst.}} = 132.5 \text{ mV}$ .

#### Zinc oxide precipitation (zinc electrode) Reaction:

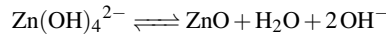

The zinc oxide precipitation reaction is a pure chemical reaction. It is modelled by the ansatz

$$j^{\text{III}} = \left(1 - \varepsilon^{\text{ZnO-L}}\right)^{\beta^{\text{ZnO-L}}} D^{\text{K}_2\text{Zn(OH)}_4} \frac{\left(c^{\text{Zn(OH)}_4^{2-}} - c^{\text{sat,Zn(OH)}_4^{2-}}\right)}{\delta^{\text{ZnO}}}, \quad (22)$$

where  $\varepsilon^{\text{ZnO-L}}$  and  $\beta^{\text{ZnO-L}}$  are the volume fraction of the porous ZnO layer and its Bruggeman coefficient regarding the pores, cf. Table S3. The saturation concentration  $c^{\text{sat,Zn(OH)}_4^{2-}}$  is found in Equation (2), and the diffusion length for the precipitation of ZnO,  $\delta^{\text{ZnO}}$ , is in the magnitude of approximately  $1 \mu\text{m}$ .

#### Primary side reactions Example reaction: OER

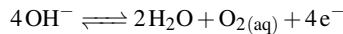

The oxygen formation is a multi-step reaction, which we do not intend to model in a precise manner here. We use a Tafel ansatz for the oxidation direction,

$$j^{\text{V}} = k^{\text{V}} \left( \frac{c^{\text{(OH)}^-}}{c^{\circ}} \right)^{4\alpha^{\text{V}}} e^{\left( (1-\alpha^{\text{V}}) \frac{z_{\text{V}}F}{RT} \eta^{\text{V}} \right)}, \quad (23)$$

with the reaction rate constant fixed at  $k^{\text{V}} = 1.50 \cdot 10^{-18} \text{ mol cm}^{-2} \text{ s}^{-1}$ ,  $\alpha^{\text{V}} = 0.5$ , the charge number  $z^{\text{V}} = 4$  and the overpotential  $\eta^{\text{V}} = \Delta\phi - \left\{ \Delta\phi^{\circ,\text{V}} + \frac{RT}{z_{\text{V}}F} \ln \left( (c^{\circ}/c^{\text{OH}^-})^4 \right) \right\}$ , with  $\Delta\phi^{\circ,\text{V}} = 0.401 \text{ V/SHE}$ . No modifications of the standard reduction potential has been made. The hydrogen formation is also modelled by a Tafel ansatz but in reduction direction. There, the reaction rate constant is chosen as  $k^{\text{IV}} = 2.50 \cdot 10^{-21} \text{ mol cm}^{-2} \text{ s}^{-1}$ ,  $\alpha^{\text{IV}} = 0.5$ , the charge number  $z^{\text{IV}} = 2$  and the overpotential  $\eta^{\text{IV}} = \Delta\phi - \left\{ \Delta\phi^{\circ,\text{IV}} + \frac{RT}{z_{\text{IV}}F} \ln \left( (c^{\circ}/c^{\text{OH}^-})^2 \right) \right\}$ , with  $\Delta\phi^{\circ,\text{IV}} = -0.828 \text{ V/SHE}$ . As we concentrate on the reduction direction, no surface concentration enters the equation in comparison to Equation 19. As before, no modification of the standard reduction potential is conducted.

**Secondary side reactions** Example reaction: oxygen recombination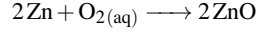

The recombination of  $\text{O}_2$  at the Zn electrode to ZnO is modelled through

$$j^{\text{VI}} = k^{\text{VI}} (c^{\text{O}_{2(\text{aq})}} - c^{\text{back}}). \quad (24)$$

As it is thought to happen fast and uni-directional,<sup>72,73</sup>  $c^{\text{back}} = 0$ . The fitted reaction rate constant is set to  $k^{\text{VI}} = 5.00 \cdot 10^{-3} \text{ s}^{-1}$ . The same approach is used to allow for outgassing to limit the amount of dissolved  $\text{H}_2$  and  $\text{O}_2$  in the electrolyte solution. The reaction rate constants are set to  $k^{\text{VII}} = 3.00 \cdot 10^2 \text{ s}^{-1}$  and  $k^{\text{VIII}} = 2.50 \cdot 10^{-1} \text{ s}^{-1}$ , respectively. The parameter  $c^{\text{back}}$  is approximated by the solubilities of the two gases in water at room temperature and atmospheric pressure,  $c^{\text{sol}, \text{H}_2(\text{aq})} = 2 \cdot 4.29 \cdot 10^{-13} \text{ mol cm}^{-3}$  and  $c^{\text{sol}, \text{O}_2(\text{aq})} = 2 \cdot 2.52 \cdot 10^{-7} \text{ mol cm}^{-3}$ , where the factor of two is used to account for disregarded influence from the gas pressure, electrolyte composition and pH value.

**Table S7** Parameters of reactions

| <b>Zinc dissolution</b>                 |                                     |                               |        |                                                                               |
|-----------------------------------------|-------------------------------------|-------------------------------|--------|-------------------------------------------------------------------------------|
| Variable                                | Unit                                | Value                         | Source | Comment                                                                       |
| $k^{\text{I}}$                          | $\text{mol cm}^{-2} \text{ s}^{-1}$ | $2.50 \cdot 10^{-10}$         | —      | fitted to experiments                                                         |
| $\alpha^{\text{I}}$                     | —                                   | 0.5                           | —      | —                                                                             |
| $z^{\text{I}}$                          | —                                   | 2                             | —      | —                                                                             |
| $\Delta\phi^{\circ, \text{I}}$          | V                                   | -1.269                        | —      | SHE; based on Ref. <sup>62</sup> with adjustments for activity and additives  |
| <b>Proton insertion</b>                 |                                     |                               |        |                                                                               |
| Variable                                | Unit                                | Value                         | Source | Comment                                                                       |
| $k^{\text{II}}$                         | $\text{mol cm}^{-2} \text{ s}^{-1}$ | $1.00 \cdot 10^{-7}$          | —      | fitted to experiments                                                         |
| $\alpha^{\text{II}}$                    | —                                   | 0.5                           | —      | —                                                                             |
| $z^{\text{II}}$                         | —                                   | 1                             | —      | —                                                                             |
| $\Delta\phi^{\circ, \text{II}}$         | V                                   | 0.365                         | —      | SHE; based on Ref. <sup>62</sup> with adjustments for activity and additives  |
| $\Delta\phi^{\text{hyst.}}$             | V                                   | 0.1325                        | —      | added when charging; chosen due to fit experimental data                      |
| <b>Zinc oxide precepitation</b>         |                                     |                               |        |                                                                               |
| Variable                                | Unit                                | Value                         | Source | Comment                                                                       |
| $\delta^{\text{ZnO}}$                   | cm                                  | $1.00 \cdot 10^{-4}$          | —      | estimated                                                                     |
| see section 3, section 4 and section 7  |                                     |                               |        |                                                                               |
| <b>Primary side reactions</b>           |                                     |                               |        |                                                                               |
| Variable                                | Unit                                | Value                         | Source | Comment                                                                       |
| $k^{\text{IV}}$                         | $\text{mol cm}^{-2} \text{ s}^{-1}$ | $2.50 \cdot 10^{-21}$         | —      | fitted to experiments                                                         |
| $\alpha^{\text{IV}}$                    | —                                   | 0.5                           | —      | —                                                                             |
| $z^{\text{IV}}$                         | —                                   | 2                             | —      | —                                                                             |
| $\Delta\phi^{\circ, \text{IV}}$         | V                                   | -0.828                        | —      | SHE; no adjustments for activity and additives                                |
| $k^{\text{V}}$                          | $\text{mol cm}^{-2} \text{ s}^{-1}$ | $1.50 \cdot 10^{-18}$         | —      | fitted to experiments                                                         |
| $\alpha^{\text{V}}$                     | —                                   | 0.5                           | —      | —                                                                             |
| $z^{\text{V}}$                          | —                                   | 4                             | —      | —                                                                             |
| $\Delta\phi^{\circ, \text{V}}$          | V                                   | 0.401                         | —      | SHE; no adjustments for activity and additives                                |
| <b>Secondary side reactions</b>         |                                     |                               |        |                                                                               |
| Variable                                | Unit                                | Value                         | Source | Comment                                                                       |
| $k^{\text{VI}}$                         | $\text{s}^{-1}$                     | $5.00 \cdot 10^{-3}$          | —      | adapted to experiments                                                        |
| $c^{\text{back}}$                       | $\text{mol cm}^{-3}$                | 0                             | —      | reaction assumed to be uni-directional                                        |
| $k^{\text{VII}}$                        | $\text{s}^{-1}$                     | $3.00 \cdot 10^2$             | —      | adapted to experiments                                                        |
| $c^{\text{sol}, \text{H}_2(\text{aq})}$ | $\text{mol cm}^{-3}$                | $2 \cdot 4.29 \cdot 10^{-13}$ | —      | two time the solubility in water at room temperature and atmospheric pressure |
| $k^{\text{VIII}}$                       | $\text{s}^{-1}$                     | $2.50 \cdot 10^{-1}$          | —      | adapted to experiments                                                        |
| $c^{\text{sol}, \text{O}_2(\text{aq})}$ | $\text{mol cm}^{-3}$                | $2 \cdot 2.52 \cdot 10^{-7}$  | —      | two time the solubility in water at room temperature and atmospheric pressure |

**10 Specific Surfaces**

The reaction rates presented in the previous section have to be multiplied by a specific surface (surface per volume) to model appropriate source terms for the volume-averaged model used in this work. For the Zn electrode we use the *geometric model* presented in Schmitt <sup>74</sup>, Sec. E.2 to calculate specific surfaces regarding the zinc particles and the zinc oxide layer, in both cases based on their respective volume fractions. For the Ni electrode the simpler *Stamm model* from the same work is used. Hence, the following set of formulas is used

to estimate the specific surfaces of the fibres and a possible zinc oxide layer.

For numerical reasons, if volume fractions approach zero, the specific surfaces are asymptotically scaled to zero.

**Geometric model (zinc particles and zinc oxide layer)** Upon initialisation, the number of Zn particles per volume,  $N^{\text{part.,Zn}}$ , is calculated based on the initial Zn volume fraction and particle radius. With this, the radii of a representative Zn particle and its ZnO layer may be calculated, which depend on the current volume fractions. Based on these, specific surfaces may be estimated for reactions happening on the Zn particle surface and on the outer surface of the ZnO layer. As usual, the  $\epsilon^s$  comprises all locally present solid phase volume fractions.

$$\begin{aligned} N^{\text{part.,Zn}} &= \frac{3}{4\pi} \frac{\epsilon^{\text{Zn},0} (1 + \epsilon^{\text{Zn},0})}{(r^{\text{Zn},0})^3} \\ r^{\text{Zn}} &= r^{\text{ZnO,i}} = \left( \frac{3}{4\pi} \frac{\epsilon^{\text{Zn}} (1 + \epsilon^{\text{Zn}})}{N^{\text{part.,Zn}}} \right)^{\frac{1}{3}} \\ r^{\text{ZnO,o}} &= \left( (r^{\text{ZnO,i}})^3 + \frac{3}{4\pi} \frac{\epsilon^{\text{ZnO}} (1 + \epsilon^{\text{ZnO}})}{\epsilon^{\text{ZnO-L}} N^{\text{part.,Zn}}} \right)^{\frac{1}{3}} \\ A^{\text{spec.,Zn}} &= N^{\text{part.,Zn}} 4\pi (r^{\text{Zn}})^2 (1 - \epsilon^s) \\ A^{\text{spec.,ZnO}} &= N^{\text{part.,Zn}} 4\pi (r^{\text{ZnO}})^2 (1 - \epsilon^s) \end{aligned} \quad (25)$$

The specific surface area  $A^{\text{spec.,Zn}}$  is relevant for the Zn dissolution and  $\text{H}_2$  formation reactions (3D: reduced  $A^{\text{spec.}}$  by a factor of 0.3 for HER),  $A^{\text{spec.,ZnO}}$  and the radii  $r^{\text{ZnO,o}}$  and  $r^{\text{ZnO,i}}$  for the ZnO precipitation reaction.

**Stamm model (nickel dihydroxide particles)** As there are no volume changes modelled in the Ni electrode, the estimation of the specific surface is of minor importance as it stays constant throughout the simulation. For the calculation, the same procedure is followed: Calculation of the number of particles per volume,  $N^{\text{part.,ca}}$ , which relies on the radius of the active particles,  $r^{\text{Ni(OH)}_2,0}$ , and based on this the estimation of the specific surface.

$$\begin{aligned} N^{\text{part.,ca}} &= \frac{3}{4\pi} \frac{\epsilon^{\text{ca},0}}{(r^{\text{Ni(OH)}_2,0})^3} \\ r^{\text{ca}} &= r^{\text{Ni(OH)}_2,0} \\ A^{\text{spec.,ca}} &= N^{\text{part.,ca}} 4\pi (r^{\text{ca}})^2 (1 - \epsilon^{\text{ca}}) \end{aligned} \quad (26)$$

$A^{\text{spec.,ca}}$  is then the relevant specific surface for the proton insertion and  $\text{O}_2$  formation reactions.

## 11 Pressure and Convection

This section treats pressure and convection in the electrolyte solution.

### 11.1 Balance Equations

The convection of the electrolyte solution, induced by pressure differences, causes a change in local liquid volume fraction  $\epsilon^l$ . As already mentioned in section 7, we use a centre-of-volume reference frame for the convection velocity  $\vec{v}$ .<sup>23,24</sup> Under the assumption of constant partial molar volumes,  $\vec{v}^k \neq \vec{v}^k(p, T, c^k)$ , the balance equation for the liquid phase volume fraction reduces to

$$\begin{aligned} \frac{\partial \epsilon^l}{\partial t} &= -\vec{\nabla} \cdot (\epsilon^l \vec{v}) + \underbrace{\sum_k \tilde{N}^{\text{v,eff},k} \cdot \vec{\nabla} (\vec{v}^k)}_{\vec{v}^k = \text{const.} \rightarrow 0} + \sum_k \vec{v}^k \left\{ \sum_r A^r v^{kr} j^r \right\} \\ &= -\vec{\nabla} \cdot (\epsilon^l \vec{v}) + \sum_k \vec{v}^k \left\{ \sum_r A^r v^{kr} j^r \right\}. \end{aligned} \quad (27)$$

Here,  $\tilde{N}^{\text{v,eff},k}$  is the effective concentration flux density in the centre-of-volume frame. Subsequently, the convection velocity is expressed through a Darcy law for multi-phase flow, which reads

$$\vec{v} = -s^l \frac{\bar{k}}{\bar{\eta}^l} \left( \vec{\nabla} (p^l) - \rho^l \vec{g} \right). \quad (28)$$

The first factor is the liquid saturation of the pore space,  $s^l = \epsilon^l / \epsilon^{\text{pore}}$ , the ratio of liquid to pore volume, accounts for the multi-phase flow character. The second one comprise the intrinsic permeability  $\bar{k}$  of the microstructure and the intrinsic dynamic viscosity of the electrolyte solution. And lastly, the convection velocity is induced by a gradient in pressure in the liquid phase,  $\vec{\nabla} (p^l)$ , and the gravitational acceleration  $\vec{g}$  time the mass density of the electrolyte solution,  $\rho^l$ .

For the calculation of the liquid phase pressure  $p^l$  a semi-empirical approach is used. The Leverett  $J$ -function<sup>75</sup> relates capillary pressure  $p^c$  to the saturation in a porous microstructure. In the present application, the capillary pressure is the difference between the pressure in the gas and liquid phase,  $p^g$  and  $p^l$ , respectively. As mentioned in section 8, we assume that  $p^g = p^{\text{atm}} = 1013.25 \text{ hPa} = \text{const.}$



stays at the atmospheric pressure and thus we reduce the capillary pressure to a difference in the liquid pressure,  $p^c = p^{\text{atm}} - (p^{\text{atm}} + \Delta p^l) = -\Delta p^l$ , as we are interested in the pressure and velocity in the liquid phase only. Lastly, we base our  $J$ -functions on the saturation of the liquid phase in pores, which gives the relation

$$p^c = p^g - p^l = -\Delta p^l = \gamma^{lg} \sqrt{\frac{\varepsilon^{\text{pore}}}{\bar{k}}} J(s^l), \quad (29)$$

where  $\gamma^{lg}$  is the surface tension of the liquid-gas interface and  $\bar{k}$ , as previously, is the intrinsic permeability of the microstructure.

For the actual shape and behaviour of the  $J$ -function little is known for typical microstructures found in components as electrodes, membranes and felts. Some works on gas diffusion electrodes<sup>76</sup> model the behaviour as the combination of two exponential functions, which was then abstracted by Schmitt *et al.*<sup>77</sup> to the combination of a sine hyperbolicus and a tangent function. A newer approach, which was successfully fitted to a wide range of applications was presented by Foroughi *et al.*,<sup>78</sup> is used here. The general form is

$$J(s^l) = \bar{A} + \bar{B} \tan\left(\frac{\pi}{2} - \pi \{s^l\}^C\right), \quad (30)$$

with constants  $\bar{A}$  (wettability-related,  $\bar{A} > 0$  for hydrophilic materials),  $\bar{B}$  (related to pore size distribution and curvature of the fluid menisci) and  $C$ , which controls the point of inflection regarding capillary pressure and the behaviour close to the limit values of  $s^l$ .

## 11.2 Material Parameters

**Permeability** The intrinsic permeability  $\bar{k}$  of the different porous structures of the electrochemical cell examined in this work are approximated and classified as follows:

- packing of spherical particles with known particle size: Zn and Ni electrodes (neglection of Ni mesh and/or other microstructures)
- packing of spherical particles with known pore size: membrane
- packing of cylindrical fibres with known fibre radius: felt

If the particle/fibre radius is used in units of cm, the permeability will have the desired unit of  $\text{cm}^2$ .

The permeability of the electrodes is estimated by the semi-empirical Kozeny-Carman equation,<sup>79–81</sup> which was modified by Schmitt *et al.*<sup>77</sup> for multi-phase flow (gas-liquid) to

$$\begin{aligned} \bar{k}^{\text{spheres}} &= \frac{\varepsilon^l}{\varepsilon^{\text{pore}}} k^{\text{KC}} \\ &= \frac{\varepsilon^l}{\varepsilon^{\text{pore}}} \frac{(\varepsilon^{\text{pore}} d)^2}{180(1 - \varepsilon^{\text{pore}})^2} \\ &= \frac{\varepsilon^l \varepsilon^{\text{pore}} d^2}{180(1 - \varepsilon^{\text{pore}})^2}, \end{aligned} \quad (31)$$

where  $d$  is the typical grain size of a solid particle (see Table S3, we assume the diameter of the Zn particle plus its ZnO shell). For the Zn electrode we note, that  $d$  may change during cycling. The typical diameter of a particle in the Ni electrode is assumed to be that of a NiO(OH)/Ni(OH)<sub>2</sub> active particle, see Table S3.

For the membrane, where often only the pore size is known and the assumption of spherical particles is far from reality, we rely on a rough estimation. Based on the hydraulic permeability found for a Celgard® 3400 membrane<sup>82</sup>, we estimate a value of about  $\bar{k}^{\text{membrane}} \approx 1 \cdot 10^{-8} \text{ cm}^2$  for a polypropylene membrane in a KOH electrolyte solution.

Lastly, for the felt, we use a semi-empirical approach for three-dimensionally and isotropically oriented long fibres given by Jackson and James<sup>83</sup>, which we modify analogously to Equation (31) for multi-phase flow:

$$\begin{aligned} \bar{k}^{\text{fibres}} &= \frac{\varepsilon^l}{\varepsilon^{\text{pore}}} \bar{k}^{\text{JJ}} \\ &= \frac{\varepsilon^l}{\varepsilon^{\text{pore}}} \frac{3r^2}{20(1 - \varepsilon^{\text{pore}})} (-\ln(1 - \varepsilon^{\text{pore}}) - 0.931) \\ &= \frac{3\varepsilon^l r^2}{20\varepsilon^{\text{pore}}(1 - \varepsilon^{\text{pore}})} (-\ln(1 - \varepsilon^{\text{pore}}) - 0.931), \end{aligned} \quad (32)$$

with  $r = r^{\text{fibre}}$  being the typical fibre radius.

**Dynamic viscosity** Based on the work of Hodges *et al.*<sup>58</sup>, the pure KOH electrolyte solution data of Klochko and Godneva,<sup>84</sup> Zaytsev and Asayev<sup>85</sup> and Guo *et al.*,<sup>86</sup> and the KOH–ZnO electrolyte solution data of Siu and Evans<sup>87</sup> and Trudgeon and Li,<sup>49</sup> we perform a curve fit which results in

$$\begin{aligned} \bar{\eta}^l &= 1 \cdot 10^{-5} \left\{ 0.8874 + 1.4426 \cdot 10^2 c^{\text{K}^+} - 1.3277 \cdot 10^4 (c^{\text{K}^+})^2 + 2.5261 \cdot 10^6 (c^{\text{K}^+})^3 \right. \\ &\quad \left. - 3.9202 \cdot 10^{-1} c^{\text{Zn(OH)}_4^{2-}} + 9.1317 \cdot 10^4 c^{\text{K}^+} c^{\text{Zn(OH)}_4^{2-}} \right\} \text{ in kg cm}^{-1} \text{ s}^{-1}, \end{aligned} \quad (33)$$

where we assumed that the dynamic viscosity of the electrolyte solution,  $\eta^l$ , is dependent on the initial hydroxide, i.e.  $\text{K}^+$ , concentration and nearly linearly dependent on  $c^{\text{Zn(OH)}_4^{2-}}$  (both in units of  $\text{mol cm}^{-3}$ ). The fixed offset is the dynamic viscosity of pure water at  $T = 25^\circ\text{C}$ . The fit has an error of about 1%.

**Mass density of the electrolyte solution** The mass density is calculated by

$$\rho^1 = \sum_k \bar{M}^k c^k, \quad (34)$$

where  $\bar{M}^k$  is the molar mass of species  $k = \{\text{H}_2\text{O}, \text{KOH}, \text{K}_2\text{Zn}(\text{OH})_4, \text{H}_2(\text{aq}), \text{O}_2(\text{aq})\}$ .

**Leverett  $J$ -function** The determination of the constants introduced in Equation 30 is based on the assumptions that the materials used in the battery cell have generally a high wettability and that, in equilibrium, the liquid-gas interface has a curvature of one. The magnitude of the values is chosen due to examples of gas diffusion electrodes presented in the work of Foroughi *et al.*<sup>78</sup>

**Table S8** Constants of the Leverett  $J$ -function.

| Component    | $\bar{A}$ | $\bar{B}$ | $C$  |
|--------------|-----------|-----------|------|
| Zn electrode | 0.20      | 0.10      | 1.00 |
| Ni electrode | 0.20      | 0.15      | 1.00 |
| Membrane     | 0.25      | 0.20      | 1.25 |
| Felt         | 0.25      | 0.10      | 1.25 |

**Surface Tension** The surface tension  $\gamma^{\text{lg}}$  between electrolyte solution and gas phase is needed to calculate the capillary pressure via the Leverett  $J$ -function. Hodges *et al.*<sup>58</sup> provide an overview of works on this surface tension for pure KOH electrolyte solutions. A wider range of weight percentage KOH (and temperatures) is covered by Feldkamp.<sup>88, Eq. 3</sup> For a simpler usage in our case, we re-fit his function for  $T = 25^\circ\text{C}$  and the use of KOH concentration. With the ansatz

$$\gamma^{\text{lg}} = 7.18 \cdot 10^{-2} - 2.58c^{\text{K}^+} + 1.32 \cdot 10^2 (c^{\text{K}^+})^{\frac{3}{2}} - 1.16 \cdot 10^3 (c^{\text{K}^+})^2 + 3.70 \cdot 10^3 (c^{\text{K}^+})^{\frac{5}{2}} \text{ in } \text{kg s}^{-2}, \quad (35)$$

the original equation is approximated with less than 1 % error in the same  $\text{K}^+$  range as the Feldkamp equation. For the simulation we neglect a dependence on the zincate concentration, and estimate the local KOH concentration through the potassium concentration in  $\text{mol cm}^{-3}$ .

**Table S9** Parameters related to convection and pressure in the electrolyte solution

| Permeability                                 |                               |                        |                                 |                                                                                                           |
|----------------------------------------------|-------------------------------|------------------------|---------------------------------|-----------------------------------------------------------------------------------------------------------|
| Variable                                     | Unit                          | Value                  | Source                          | Comment                                                                                                   |
| $\bar{k}_{\text{spheres}}$                   | $\text{cm}^2$                 | (31)                   | Ref. <sup>79–81</sup>           | adapted for multi-phase flow; used in Zn and Ni electrode and the membrane with respective radii          |
| $\bar{k}_{\text{fibres}}$                    | $\text{cm}^2$                 | (32)                   | Ref. <sup>83</sup>              | adapted for multi-phase flow; used in the felt                                                            |
| $\bar{k}_{\text{membrane}}$                  | $\text{cm}^2$                 | $1 \cdot 10^{-8}$      | Ref. <sup>82</sup>              | hydraulic permeability found for Celgard® 3400 membrane                                                   |
| Dynamic viscosity                            |                               |                        |                                 |                                                                                                           |
| Variable                                     | Unit                          | Value                  | Source                          | Comment                                                                                                   |
| $\bar{\eta}^1$                               | $\text{kg cm}^{-1} \text{s}$  | (33)                   | Ref. <sup>49,58,87</sup>        | own fit for $T = 25^\circ\text{C}$                                                                        |
| Mass density                                 |                               |                        |                                 |                                                                                                           |
| Variable                                     | Unit                          | Value                  | Source                          | Comment                                                                                                   |
| $\rho^1$                                     | $\text{kg cm}^{-3}$           | (34)                   | —                               | —                                                                                                         |
| Molar masses                                 |                               |                        |                                 |                                                                                                           |
| Variable                                     | Unit                          | Value                  | Source                          | Comment                                                                                                   |
| $\bar{M}^{\text{H}_2\text{O}}$               | $\text{kg mol}^{-1}$          | $18.02 \cdot 10^{-3}$  | —                               | —                                                                                                         |
| $\bar{M}^{\text{KOH}}$                       | $\text{kg mol}^{-1}$          | $56.12 \cdot 10^{-3}$  | —                               | —                                                                                                         |
| $\bar{M}^{\text{K}_2\text{Zn}(\text{OH})_4}$ | $\text{kg mol}^{-1}$          | $211.61 \cdot 10^{-3}$ | —                               | —                                                                                                         |
| $\bar{M}^{\text{H}_2(\text{aq})}$            | $\text{kg mol}^{-1}$          | $2.02 \cdot 10^{-3}$   | —                               | —                                                                                                         |
| $\bar{M}^{\text{O}_2(\text{aq})}$            | $\text{kg mol}^{-1}$          | $32.00 \cdot 10^{-3}$  | —                               | —                                                                                                         |
| Partial molar volumes                        |                               |                        |                                 |                                                                                                           |
| Variable                                     | Unit                          | Value                  | Source                          | Comment                                                                                                   |
| $\bar{v}^{\text{H}_2\text{O}}$               | $\text{cm}^3 \text{mol}^{-1}$ | 17.27                  | Ref. <sup>89</sup> , Sec. D.1.4 | evaluated for initial concentrations (cf. Table S4); $c^{\text{H}_2\text{O}} = 0.048 \text{ mol cm}^{-3}$ |
| $\bar{v}^{\text{KOH}}$                       | $\text{cm}^3 \text{mol}^{-1}$ | 20.21                  | Ref. <sup>89</sup> , Sec. D.1.4 | evaluated for initial concentrations (cf. Table S4); $c^{\text{H}_2\text{O}} = 0.048 \text{ mol cm}^{-3}$ |
| $\bar{v}^{\text{K}_2\text{Zn}(\text{OH})_4}$ | $\text{cm}^3 \text{mol}^{-1}$ | 73.76                  | Ref. <sup>89</sup> , Sec. D.1.4 | evaluated for initial concentrations (cf. Table S4); $c^{\text{H}_2\text{O}} = 0.048 \text{ mol cm}^{-3}$ |
| $\bar{v}^{\text{H}_2(\text{aq})}$            | $\text{cm}^3 \text{mol}^{-1}$ | 26.7                   | Ref. <sup>90</sup>              | at infinite dilution in water                                                                             |

|                                         |                                   |                      |                                             |                                                                           |
|-----------------------------------------|-----------------------------------|----------------------|---------------------------------------------|---------------------------------------------------------------------------|
| $\bar{v}^{\text{O}_2(\text{aq})}$       | $\text{cm}^3 \text{mol}^{-1}$     | 33.2                 | Ref. <sup>90</sup>                          | at infinite dilution in water                                             |
| <b>Leverett <math>J</math>-function</b> |                                   |                      |                                             |                                                                           |
| <b>Variable</b><br>see Table S8         | <b>Unit</b>                       | <b>Value</b>         | <b>Source</b>                               | <b>Comment</b>                                                            |
| <b>Surface tension</b>                  |                                   |                      |                                             |                                                                           |
| <b>Variable</b><br>$\gamma^{\text{lg}}$ | <b>Unit</b><br>$\text{kg s}^{-2}$ | <b>Value</b><br>(35) | <b>Source</b><br>Ref. <sup>88</sup> , Eq. 3 | <b>Comment</b><br>re-fit for $T = 25^\circ\text{C}$ and KOH concentration |

## 12 Auxiliary Results

### 12.1 Parameter sensitivity

In the article we have seen that there are processes such as the OER that have a visible influence on the general cell behaviour. Most of these processes are related to the material parameters listed in Table 1 of the article, which may assume values in a certain range due to their dependence on, for example, the additives used. It is therefore worth investigating how a modification of the processes mentioned affects the behaviour of the cell. To this end, we vary the tabulated parameters in this section in order to evaluate the effect and significance for the behaviour of the cell.

The procedure is as follows: Starting from the base scenario, which is the third formation cycle as used in the other simulations, we change each of the parameters found in Table 1 of the article individually in both directions, i.e. to make the process stronger and weaker. For some parameters, where it showed that a variation in one of the directions does not have a visible influence, only the other one is examined. Generally, as the currents in the formation cycles are relatively low, the variations have to be chosen rather large for a significant effect.

In the following, the parameter variations are examined in pairs and are depicted in the respective panel in Figure S7, where the grey curve always represents the base scenario.

**Main reactions** Figure S7a illustrates reaction rate constants  $k^{\text{I}}$  and  $k^{\text{II}}$  for the main reactions. Reducing  $k^{\text{I}}$  for Zn dissolution symmetrically increases the spread between charge-discharge branches parallel to the base curve. Decreasing  $k^{\text{II}}$  for proton insertion primarily shifts the discharge branch downward while altering the slope in the charging branch giving a higher cell voltage at the beginning, which gradually fades away towards the end of charge.

These behaviours result from interactions between main and side reactions at both electrodes. Lower rate constants require higher overpotentials to maintain current, creating the observed spreads. For  $k^{\text{I}}$ , effects appear uniform because HER operates consistently throughout cycling. For  $k^{\text{II}}$ , OER dominates the Ni electrode toward charge completion, driving convergence of cell voltage. During discharge, OER inactivity produces parallel voltage shifts proportional to overpotential. Higher charging overpotentials activate OER earlier, extracting fewer protons from Ni particles, which manifests as earlier voltage drops during discharge.

**Side reactions** Figure S7b demonstrates the effects of rate constants  $k^{\text{IV}}$  and  $k^{\text{V}}$  for HER and OER. HER requires extreme amplification to produce visible effects, yielding minimal impact on charging and only slight discharge shifts. Conversely, OER generates significant voltage changes with minor constant variations, where stronger OER lowers the end-of-charge plateau and shortens discharge operation, while weaker OER produces opposite effects.

HER's minimal influence stems from its substantially slower kinetics compared to Zn dissolution (cf. Table 1 of the article). During discharge, where overpotentials of the two reactions at the Zn electrode are in a more similar range, HER concentration overpotential marginally affects end-of-discharge voltage drop. In contrast, OER's  $k^{\text{V}}$  significantly impacts cell voltage through the onset of end-of-charge plateau via its overpotential and the increasing SOC-based OCP curve of the proton insertion reaction (see Equation (21)). This directly modulates proton extraction from active particles, consequently affecting discharge capacity. While rate constant changes scale reaction overpotentials, explaining discharge branch voltage shifts, the charge branch remains largely stable because HER is inherently weak and OER becomes significant only at higher SOC. Notably,  $k^{\text{IV}}$  (HER) influence remains negligible due to cell design ensuring  $\text{H}_2$  production inferior to  $\text{O}_2$  production.

**Solid diffusion constants** Figure S7c shows the impact of proton solid diffusion constants  $D^{\text{NiO(OH)}}$  and  $D^{\text{Ni(OH)}_2}$  in  $\text{NiO(OH)/Ni(OH)}_2$  particles. Reduced  $D^{\text{NiO(OH)}}$  increases mid-charging voltage with a steeper slope, followed by a second voltage rise at charge completion, while decreasing discharged capacity. Conversely,  $D^{\text{Ni(OH)}_2}$  variations produce minimal effects, showing only slight changes at charge initiation or discharge termination.

Analysis of the weighted diffusion coefficient (see (7)) reveals  $D^{\text{NiO(OH)}}$  rapidly becomes dominant with increasing SOC. During charging, lower  $D^{\text{NiO(OH)}}$  impedes proton diffusion from particle centre to the outer shell at mid-to-high SOC, depleting outer shell protons prematurely. This alters the OCP curve (see Equation (21)) of the proton insertion reaction, elevating cell voltage. At a certain SOC, OER dominance creates a voltage plateau, but continued extraction with retarded diffusion severely depletes outer shell protons, causing exponential OCP growth. This earlier onset reduces discharge capacity — a condition exacerbated by slow diffusion from outer shell to centre, which increases outer shell proton concentration and triggers exponential OCP decay.  $D^{\text{Ni(OH)}_2}$  influences only at extremely low SOC, with effects potentially diminished by coarse particle resolution (five grid points) and model sensitivity only at rarely-reached low SOC states.

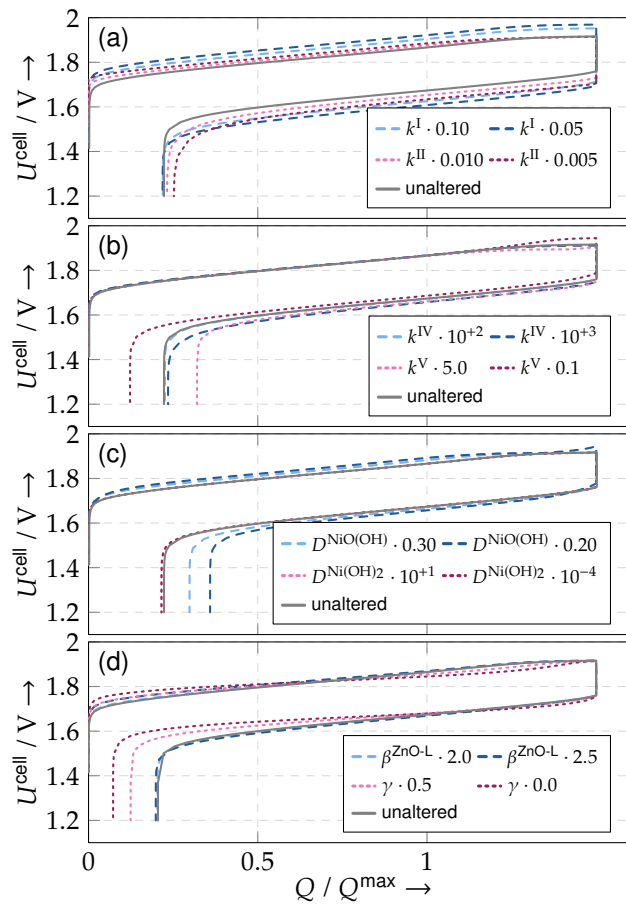

**Figure S7** Influence of fitting parameters on the cell voltage during charge/discharge. (a) Reaction rate constants  $k^I$  and  $k^{II}$ . (b) Reaction rate constants  $k^{IV}$  and  $k^V$ . (c) Solid diffusion coefficients  $D^{\text{NiO(OH)}}$  and  $D^{\text{Ni(OH)}_2}$ . (d) Bruggeman coefficient  $\beta^{\text{ZnO-L}}$  and OCP interaction coefficient  $\gamma$ . For the simulations, the formation cycle protocol is used and the third cycle is shown.

**Zinc oxide layer and nickel electrode's OCP** Figure S7d examines the Bruggeman coefficient in ZnO layer pores,  $\beta^{\text{ZnO-L}}$ , and interaction coefficient  $\gamma$  affecting the linear segment of the proton insertion reaction OCP curve (see Equation (21)). Increased  $\beta^{\text{ZnO-L}}$  elevates cell voltage at the beginning of charging before converging with the base scenario at charge completion, while lowering cell voltage slightly during discharge. Reduced  $\gamma$  substantially modifies voltage curve morphology, flattening both branches and accentuating OCP logarithmic character, maintaining the level of the end-of-charge voltage plateau but delaying final discharge voltage drop.

The Bruggeman coefficient  $\beta^{\text{ZnO-L}}$  modulates ion transport through the ZnO layer surrounding Zn particles. At lower SOC, thicker layers restrict transport, limiting available ions at the zinc surface, thereby increasing overpotential and cell voltage. A behaviour which becomes more pronounced when  $\beta^{\text{ZnO-L}}$  and hence the tortuosity is increased. As the ZnO layer dissolves at higher SOC, voltage returns to its base scenario. Meanwhile,  $\gamma$  governs the OCP linear segment slope near SOC = 0.5. Decreasing  $\gamma$  weakens the linear component, symmetrically flattening the curve and emphasising exponential extremes. Consequently, the proton insertion reaction's overpotential generates higher voltage at lower SOC and reduced voltage at higher SOC. This extended low-overpotential phase at high SOC diminishes OER activity, enabling higher capacity evident in the discharge curve.

## 12.2 Shape change

To give a more detailed analysis of the zinc shape change, the elemental Zn distribution of Figure 9 of the article is split to its contributions stemming from metallic Zn and ZnO, see Figure S8.

## Notes and references

- [1] B. Doppl, F. K. Schwab, N. J. Herrmann and B. Horstmann, *Modeling the influence of zinc particle size on gas evolution in secondary nickel-zinc battery cells*, to be submitted.
- [2] SunErgy, *private communication*, unpublished.
- [3] SunErgy, *private communication*, unpublished.
- [4] M.-B. Liu, G. M. Cook and N. P. Yao, *Journal of The Electrochemical Society*, 1981, **128**, 1663.

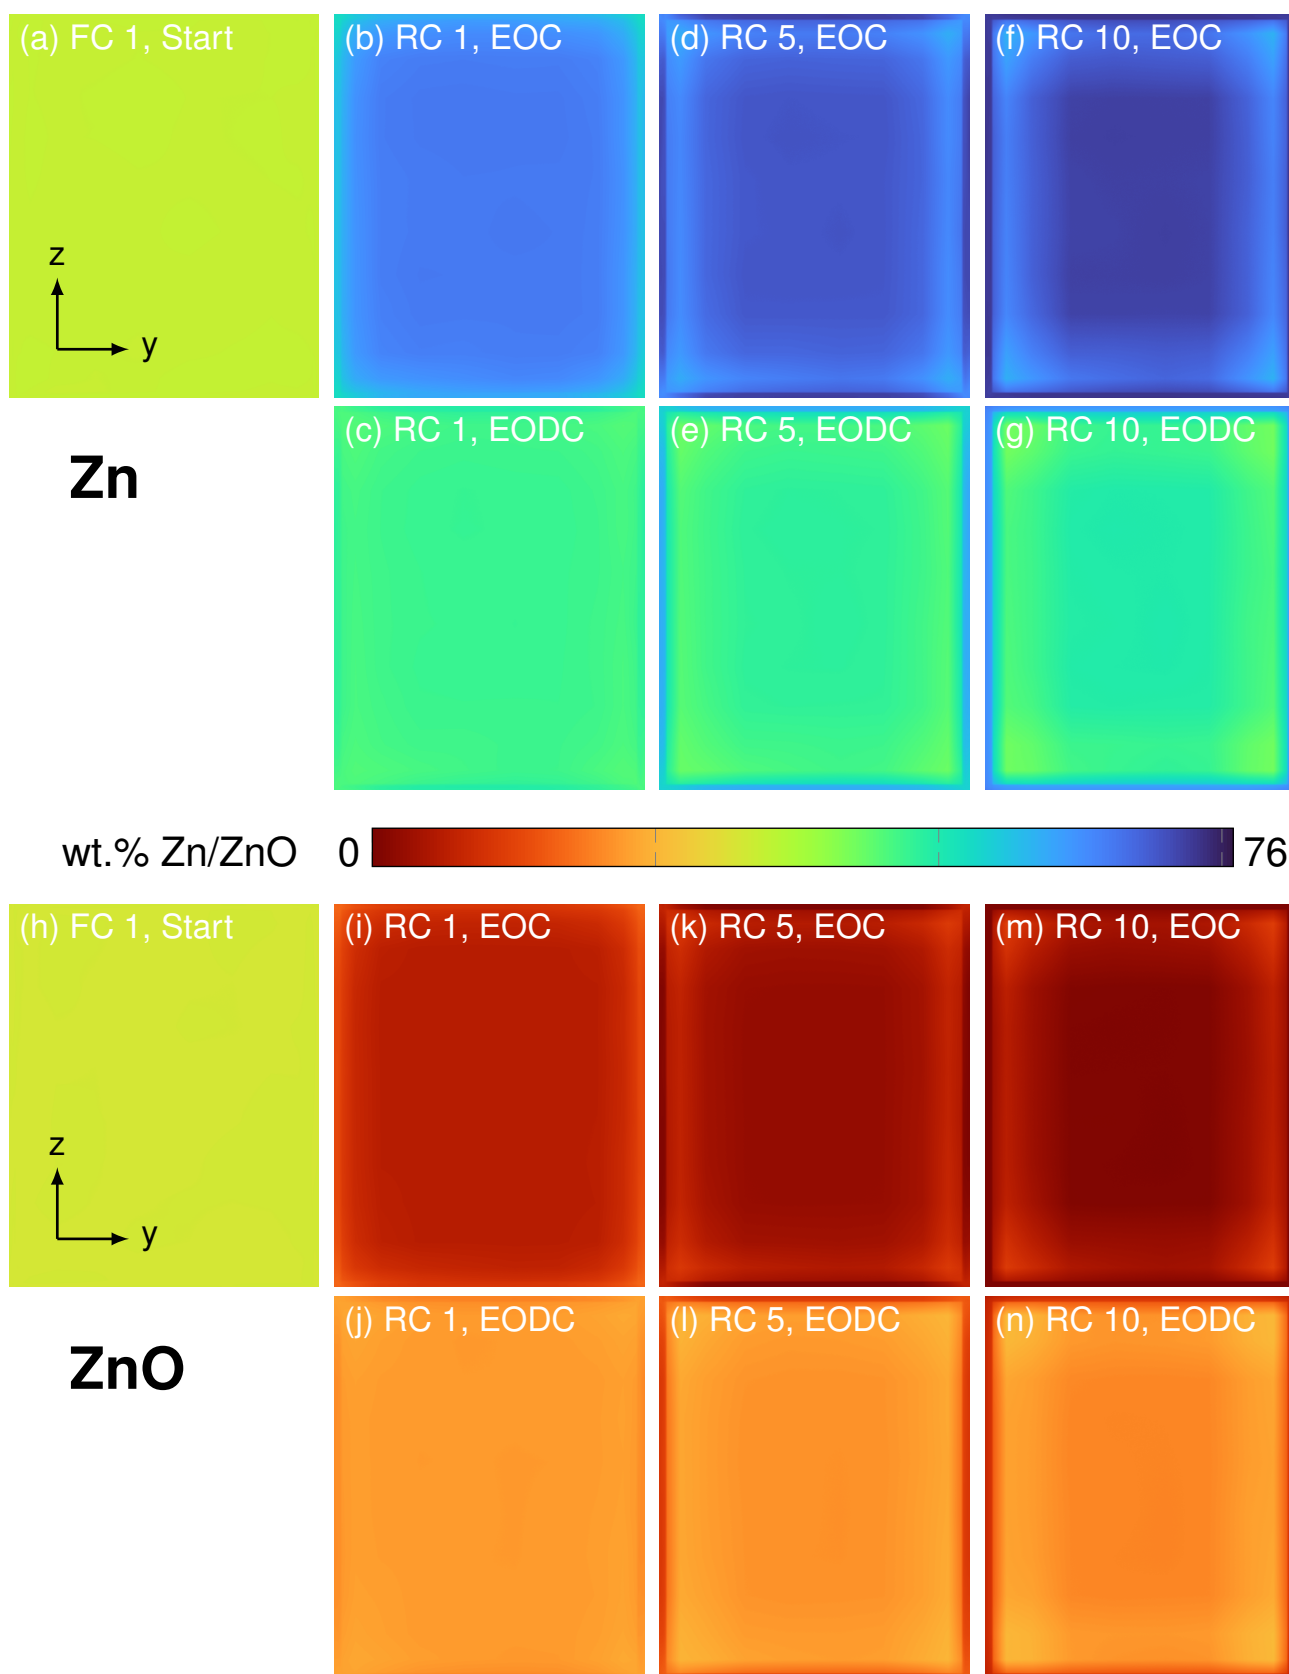

**Figure S8** Zn and ZnO distribution in virtual cell. (a) and (h) show the initial distribution of Zn/ZnO in weight percent. (b) to (g) and (i) to (n) depict the backside of the virtual Zn electrode at end of charge (EOC) and end of discharge (EODC) at different cycles and for Zn and ZnO, respectively.

- [5] Q. C. Horn and Y. Shao-Horn, *Journal of The Electrochemical Society*, 2003, **150**, A652.
- [6] ZSW, *private communication*, unpublished.
- [7] Cergy Paris Université, *private communication*, unpublished.
- [8] J. Blazy and R. Blazy, *Case Studies in Construction Materials*, 2021, **14**, e00549.
- [9] W. G. Sunu, *PhD thesis*, University of California, Los Angeles, CA, 1978.
- [10] E. J. Podlaha and H. Y. Cheh, *Journal of The Electrochemical Society*, 1994, **141**, 15.
- [11] Z. Mao and R. E. White, *Journal of The Electrochemical Society*, 1992, **139**, 1105.
- [12] J. Kriegsmann and H. Cheh, *Journal of Power Sources*, 1999, **84**, 52–62.
- [13] K. Takahashi, *Corrosion Engineering*, 1974, **23**, 557–572.
- [14] P. H. Miller, *Phys. Rev.*, 1941, **60**, 890–895.
- [15] H. O. Pierson, *Handbook of Refractory Carbides and Nitrides: Properties, Characteristics, Processing, and Applications*, Noyes Publications, Westwood, NJ, 1996, p. 362.
- [16] V. G. Orlov, A. A. Bush, S. A. Ivanov and V. V. Zhurov, *Journal of Low Temperature Physics*, 1996, **105**, 1541–1546.
- [17] F. Freund and H. Wengeler, *Berichte der Bunsengesellschaft für physikalische Chemie*, 1980, **84**, 866 – 873.
- [18] Y. Nishi, S. Iizuka, M. C. Faudree and R. Oyama, *MATERIALS TRANSACTIONS*, 2012, **53**, 940–945.
- [19] V. Srinivasan, J. W. Weidner and R. E. White, *Journal of Solid State Electrochemistry*, 2000, **4**, 367–382.
- [20] S. Motupally, C. C. Streinz and J. W. Weidner, *Journal of The Electrochemical Society*, 1995, **142**, 1401.
- [21] R. A. Matula, *Journal of Physical and Chemical Reference Data*, 1979, **8**, 1147–1298.
- [22] G. T. Meaden, *Electrical Resistance of Metals*, Springer US, Boston, MA, 1965, pp. XV, 218.
- [23] M. Schammer, B. Horstmann and A. Latz, *Journal of The Electrochemical Society*, 2021, **168**, 026511.
- [24] F. Kilchert, M. Lorenz, M. Schammer, P. Nürnberg, M. Schönhoff, A. Latz and B. Horstmann, *Phys. Chem. Chem. Phys.*, 2023, **25**, 25965–25978.
- [25] A. Latz and J. Zausch, *Journal of Power Sources*, 2011, **196**, 3296–3302.
- [26] A. Katchalsky and P. F. Curran, *Nonequilibrium Thermodynamics in Biophysics*, Harvard University Press, Cambridge, MA and London, England, 1965.
- [27] K. D. Fong, H. K. Bergstrom, B. D. McCloskey and K. K. Mandadapu, *AIChE Journal*, 2020, **66**, e17091.
- [28] B. Paxton and J. Newman, *Journal of The Electrochemical Society*, 1997, **144**, 3818.
- [29] R. N. Bhatia, K. E. Gubbins and R. D. Walker, *Trans. Faraday Soc.*, 1968, **64**, 2091–2099.
- [30] D. M. See and R. E. White, *Journal of Chemical & Engineering Data*, 1998, **43**, 986–988.
- [31] J. McBreen, *Study to investigate and improve the zinc electrode for spacecraft electrochemical cells*, Yardney Electric Corp. New York Contractor Report NASA-CR-92599, 1967.
- [32] L. Nanis, *Study of zinc-silver oxide battery system*, California Institute of Technology Contractor Report NASA-CR-109347, 1970.
- [33] T. P. Dirkse, *Power Sources 3; Research and Development in Non-mechanical Electrical Power Sources: Proceedings of the 7th International Symposium*, Newcastle upon Tyne, UK, 1970, pp. 485–493.
- [34] J. L. Gendler, *Master's thesis*, University of Pennsylvania, Philadelphia, PA, 1976.
- [35] S. U. Falk and A. J. Salkind, *Alkaline Storage Batteries*, John Wiley & Sons, New York, NY, 1969, p. 656.
- [36] K. W. Choi and N. P. Yao, *Proceedings of the Symposium on Battery Design and Optimization*, Princeton, NJ, 1979, pp. 62–80.
- [37] M. J. Isaacson, F. R. McLarnon and E. J. Cairns, *Journal of The Electrochemical Society*, 1990, **137**, 2014.
- [38] J. Chen and H. Y. Cheh, *Journal of The Electrochemical Society*, 1993, **140**, 1205.

- [39] C. E. May and H. E. Kautz, Technical Report at 154th Electrochemical Society Meeting, 1978, p. 20.
- [40] W. H. Dyson, L. A. Schreier, W. P. Sholette and A. J. Salkind, *Journal of The Electrochemical Society*, 1968, **115**, 566.
- [41] M. Liu, B. R. Faulds, G. M. Cook and N. P. Yao, *Journal of The Electrochemical Society*, 1981, **128**, 2049.
- [42] D. Trudgeon, *PhD thesis*, University of Exeter, Exeter, UK, 2019.
- [43] M. I. Usanovich and T. I. Sushkevich, *Zhurnal Prikladnoy Khimii [Journal of Applied Chemistry]*, 1951, **24**, 590–592.
- [44] D. N. Bennion, *PhD thesis*, University of California, Berkeley, CA, 1964.
- [45] V. Yushkevich, I. Maksimova and V. Bullan, *Elektrokhimiya*, 1967, **3**, 1491–1493.
- [46] H. J. De Wane and W. J. Hamer, *Electrochemical data. Part 10 - Electrolytic conductivity of aqueous solutions of the alkali metal hydroxides*, National Bureau of Standards Washington Contractor Report NASA-CR-97593, 1968.
- [47] D. M. See and R. E. White, *Journal of Chemical & Engineering Data*, 1997, **42**, 1266–1268.
- [48] R. Gilliam, J. Graydon, D. Kirk and S. Thorpe, *International Journal of Hydrogen Energy*, 2007, **32**, 359–364.
- [49] D. P. Trudgeon and X. Li, *Electrochimica Acta*, 2021, **367**, 137479.
- [50] A. A. Lang, *PhD thesis*, University of Western Ontario, London, ON, Canada, 1956.
- [51] A. Himy, *Silver-Zinc Battery: Phenomena and Design Principles*, Vantage Press, Inc., New York, NY, 1986, p. 79.
- [52] G. Akerlof and P. Bender, *Journal of the American Chemical Society*, 1941, **63**, 1085–1088.
- [53] A. Kube, N. Wagner and K. A. Friedrich, *Journal of The Electrochemical Society*, 2021, **168**, 050531.
- [54] S. Lengyel, J. Giber, G. Beke and A. Vértes, *Acta Chim. Hung. Tomus*, 1963, **39**, 357–364.
- [55] E. L. Cussler, *Diffusion: Mass Transfer in Fluid Systems*, Cambridge University Press, Cambridge, UK, 2009, p. 647.
- [56] J. Newman and N. P. Balsara, *Electrochemical systems*, Wiley, Hoboken, NJ, 4th edn, 2021.
- [57] M. J. Tham, R. D. J. Walker and K. E. Gubbins, *The Journal of Physical Chemistry*, 1970, **74**, 1747–1751.
- [58] A. Hodges, S. Renz, F. Lohmann-Richters, A. Al-Musawi, A. Jupke, W. Lehnert, G. F. Swiegers and G. G. Wallace, *Journal of Chemical & Engineering Data*, 2023, **68**, 1485–1506.
- [59] J. Stamm, A. Varzi, A. Latz and B. Horstmann, *Journal of Power Sources*, 2017, **360**, 136–149.
- [60] J. O. Bockris, Z. Nagy and A. Damjanovic, *Journal of The Electrochemical Society*, 1972, **119**, 285.
- [61] A. J. Bard and L. R. Faulkner, *Electrochemical Methods: Fundamentals and Applications*, John Wiley & Sons, New York, NY, 2nd edn, 2000.
- [62] *CRC Handbook of Chemistry and Physics*, ed. D. R. Lide, CRC Press, Boca Raton, FL, 85th edn, 2005.
- [63] J. Hendrikx, A. van der Putten, W. Visscher and E. Barendrecht, *Electrochimica Acta*, 1984, **29**, 81–89.
- [64] R. Jain, T. C. Adler, F. R. McLarnon and E. J. Cairns, *Journal of Applied Electrochemistry*, 1992, **22**, 1039–1048.
- [65] K. Malaie, F. Scholz and U. Schröder, *ChemElectroChem*, 2023, **10**, e202201118.
- [66] K. Watanabe and N. Kumagai, *Journal of Power Sources*, 1997, **66**, 121–127.
- [67] K. Watanabe and N. Kumagai, *Journal of Power Sources*, 1998, **76**, 167–174.
- [68] P. Atkins and J. de Paula, *Atkins' Physical Chemistry*, W. H. Freeman and Company, New York, NY, 8th edn, 2006, p. 1096.
- [69] K. P. Ta and J. Newman, *Journal of The Electrochemical Society*, 1999, **146**, 2769.
- [70] V. Srinivasan, J. W. Weidner and J. Newman, *Journal of The Electrochemical Society*, 2001, **148**, A969.
- [71] P. Albertus, J. Christensen and J. Newman, *Journal of The Electrochemical Society*, 2007, **155**, A48–A60.
- [72] J. Jindra, *Journal of Power Sources*, 1992, **37**, 297–313.
- [73] T. B. Reddy, *Linden's Handbook of Batteries*, McGraw-Hill Education, New York, NY, 4th edn, 2010.

- [74] T. Schmitt, *PhD thesis*, University of Ulm, Ulm, Germany, 2020.
- [75] M. Leverett, *Transactions of the AIME*, 1941, **142**, 152–169.
- [76] T. Danner, B. Horstmann, D. Wittmaier, N. Wagner and W. G. Bessler, *Journal of Power Sources*, 2014, **264**, 320–332.
- [77] T. Schmitt, T. Arlt, I. Manke, A. Latz and B. Horstmann, *Journal of Power Sources*, 2019, **432**, 119–132.
- [78] S. Foroughi, B. Bijeljic and M. J. Blunt, *Transport in Porous Media*, 2022, **145**, 683–696.
- [79] J. Kozeny, *Sitzungsberichte der Akademie der Wissenschaften mathematisch-naturwissenschaftliche Klasse*, 1927, **136**, 271–306.
- [80] P. Carman, *Transactions of the Institution of Chemical Engineers*, 1937, **15**, 150–156.
- [81] J. Bear, *Dynamics of Fluids in Porous Media*, Dover Publications, New York, NY, 1972, p. 1729.
- [82] R. S. Yeo, *Research on separators for alkaline zinc batteries: Final report*, Pinnacle Research Institute Contractor Report AC03-76SF00098, 1985.
- [83] G. W. Jackson and D. F. James, *The Canadian Journal of Chemical Engineering*, 1986, **64**, 364–374.
- [84] M. A. Klochko and M. M. Godneva, *Zhurnal Neorganicheskoi Khimii (Journal of Inorganic Chemistry)*, 1959, **4**, 2127–2135.
- [85] I. D. Zaytsev and G. G. Asayev, *Properties of Aqueous Solutions of Electrolytes*, CRC Press, Boca Raton, FL, 1992, p. 1729.
- [86] Y. jie Guo, H. bin Xu, F. Guo, S. li Zheng and Y. Zhang, *Transactions of Nonferrous Metals Society of China*, 2010, **20**, s32–s36.
- [87] S. Siu and J. W. Evans, *Journal of The Electrochemical Society*, 1997, **144**, 1278.
- [88] K. Feldkamp, *Chemie Ingenieur Technik*, 1969, **41**, 1181–1183.
- [89] T. Schmitt, A. Latz and B. Horstmann, *Electrochimica Acta*, 2020, **333**, 135491.
- [90] J. C. Moore, R. Battino, T. R. Rettich, Y. P. Handa and E. Wilhelm, *Journal of Chemical & Engineering Data*, 1982, **27**, 22–24.
